# Supplementary material for: Learning to Score Behaviors for Guided Policy Optimization
Source: arXiv:1906.04349 source file (2020-03-04)
Supplement: Supplementary file 1 [file old_appendix_theory.tex]

 
\begin{comment}
\subsection{Random features stochastic gradients}

For this and the following sections we will make use of the following expression:

    \begin{align}
    F(\theta, \mathbf{p}^{\lambda_{\pi_{\theta}}}, \mathbf{p}^{\lambda_{\pi^{\prime}}}) &= \beta \int_{\Gamma} \left( \mathbf{p}^{\lambda_{\pi'}}  \right)^\top \Phi(\tau(\pi')) d \tau(\pi') + \beta \int_{\Gamma} \left(  \mathbf{p}^{\lambda_\theta}   \right)^\top \Phi( \tau(\pi_\theta) ) d\tau(\pi_\theta)   - \label{equation::random_features_objective}  \\
    & \gamma \beta \int_{\Gamma \times \Gamma} \exp\left(.  \frac{ \left(\mathbf{p}^{\lambda_{\pi'} }   \right)^\top \Phi(\tau(\pi')) + \left(  \mathbf{p}^{\lambda_{\pi_\theta}}  \right)^\top \Phi(\tau(\pi_\theta)) - C(\Phi( \tau(\pi')), \Phi(\tau(\pi_\theta) ))  }{\gamma}      \right) d \tau(\pi') d\tau(\pi_\theta) \notag
\end{align}

We now prove the following Lemma:

\begin{lemma}
\label{imp-lemma_appendix}
The gradient $\nabla_{\mathbf{p}^{\lambda_{\pi_{\theta}}}} F(\theta, \mathbf{p}^{\lambda_{\pi_{\theta}}}, \mathbf{p}^{\lambda_{\pi^{\prime}}})$
of the objective function from Equation \ref{equation::random_features_objective} with respect to parameters  $\mathbf{p}^{\lambda_{\pi_{\theta}}}$ satisfies for $T=\exp\left(           \frac{ (\mathbf{p}^{\lambda_{\pi_{\theta}}})^{\top}\Phi(\tau_{1}) + (\mathbf{p}^{\lambda_{\pi^{\prime}}})^{\top}\Phi(\tau_{2}) - C(\Phi(\tau_{1}),\Phi(\tau_{2}))  }{   \gamma }     \right)$:
\begin{align}
\begin{split}
    \nabla_{\mathbf{p}^{\lambda_{\pi_{\theta}}}} F(\theta, \mathbf{p}^{\lambda_{\pi_{\theta}}}, \mathbf{p}^{\lambda_{\pi^{\prime}}})
    = \beta \mathbb{E}_{(\tau_{1},\tau_{2}) \sim \pi_{\theta} \bigotimes \pi^{\prime}}\left[ \Phi(\tau_{1}) - T   \Phi(\tau_{1})   \right],
\end{split}    
\end{align}
and an analogous result holds for $\nabla_{\mathbf{p}^{\lambda_{\pi^{\prime}}}} F(\theta, \mathbf{p}^{\lambda_{\pi_{\theta}}}, \mathbf{p}^{\lambda_{\pi^{\prime}}})$.
\end{lemma}

\begin{proof}
Note that the objective function from Equation \ref{maxmax} is of the form:
\begin{align*}
    F(\theta, \mathbf{p}^{\lambda_{\pi_{\theta}}}, \mathbf{p}^{\lambda_{\pi^{\prime}}}) = \beta \int_{\Gamma} \left( \mathbf{p}^{\lambda_{\pi'}}  \right)^\top \Phi(\tau(\pi')) d \tau(\pi') + \beta \int_{\Gamma} \left(  \mathbf{p}^{\lambda_\theta}   \right)^\top \Phi( \tau(\pi_\theta) ) d\tau(\pi_\theta)   - \\
    \gamma \beta \int_{\Gamma \times \Gamma} \exp\left(.  \frac{ \left(\mathbf{p}^{\lambda_{\pi'} }   \right)^\top \Phi(\tau(\pi')) + \left(  \mathbf{p}^{\lambda_{\pi_\theta}}  \right)^\top \Phi(\tau(\pi_\theta)) - C(\Phi( \tau(\pi')), \Phi(\tau(\pi_\theta) ))  }{\gamma}      \right) d \tau(\pi') d\tau(\pi_\theta) 
\end{align*}
And therefore:
\begin{align*}
\begin{split}
   \nabla_{\mathbf{p}^{\lambda_{\pi_{\theta}}}} F(\theta, \mathbf{p}^{\lambda_{\pi_{\theta}}}, \mathbf{p}^{\lambda_{\pi^{\prime}}}) =  \beta \int_{\Gamma}  \Phi( \tau(\pi_\theta) ) d\tau(\pi_\theta)   - 
     \beta \int_{\Gamma \times \Gamma} T \Phi(\tau(\pi_\theta)) d \tau(\pi') d\tau(\pi_\theta), 
\end{split}
\end{align*}
where $T=\exp\left( \frac{ \left(\mathbf{p}^{\lambda_{\pi'} }   \right)^\top \Phi(\tau(\pi')) + \left(  \mathbf{p}^{\lambda_{\pi_\theta}}  \right)^\top \Phi(\tau(\pi_\theta)) - C(\Phi( \tau(\pi')), \Phi(\tau(\pi_\theta) ))  }{\gamma}      \right)$.
Rewriting this expression in terms of expectations gives:
\begin{align}
\begin{split}
    \nabla_{\mathbf{p}^{\lambda_{\pi_{\theta}}}} F(\theta, \mathbf{p}^{\lambda_{\pi_{\theta}}}, \mathbf{p}^{\lambda_{\pi^{\prime}}})
    = \beta \mathbb{E}_{(\tau_{1},\tau_{2}) \sim \pi_{\theta} \bigotimes \pi^{\prime}}\left[ \Phi(\tau_1) - T   \Phi(\tau_1)   \right],
\end{split}    
\end{align}
and that completes the proof.



\end{proof}





\end{comment}




 
 
 
 
 
 \subsection{BGPG, BGES and their theoretical guarantees}
 
Here we provide some theoretical guarantees for our algorithms. Both proposed methods BGPG and BGES follow the alternating optimization algorithmic template. We start by noting that stripped to their bare bones components our algorithms satisfy two paradigms:
\begin{enumerate}
    \item Min-Max optimization. When $\beta < 0$ the algorithms we propose for solving the optimization objective in Equation \label{eq:rlobj}, turn into an Alternating Min-Max optimization procedure. Henceforth whenever we refer to the problem defined by setting $\beta<0$ we will call it the Min-Max problem.   
    \item Max-Max optimization. When $\beta > 0$ the algorithms we propose for solving the optimization objective in Equation \label{eq:rlobj} turn into an alternating Max-Max procedure. Henceforth whenever we refer to the problem defined by setting $\beta<0$ we will call it the Max-Max problem.   
\end{enumerate}

Our theoretical results will therefore center around providing guarantees for optimizing an objective of the form:

\begin{align}
    F(\theta, \mathbf{p}^{\pi_\theta}, \mathbf{p}^{\pi'}) &= \mathbb{E}_{\tau_1, \tau_2 \sim \mathbb{P}_{\pi_\theta} \bigotimes \mathbb{P}_{ \pi' } }\Big[ \mathcal{R}(\pi_1) + \langle \mathbf{p}^{\pi_\theta}, \phi_\kappa( \Phi(\tau_1)) \rangle - \beta \langle \mathbf{p}^{\pi'}, \phi_\kappa(\Phi(\tau_2) ) \rangle  + \label{equation::theory_objective} \\
    &\quad\gamma \beta \exp\left( \frac{ \langle \mathbf{p}^{\pi_\theta}, \phi_\kappa(\Phi(\tau_1))    \rangle - \langle   \phi^{\pi'}, \phi_\kappa(\Phi(\tau_2))       \rangle - C( \Phi(\tau_1), \Phi(\tau_2)  )      }{\gamma}           \right) 
    \Big]\notag
\end{align}

Where $\pi_\theta$ is a policy parametrized by $\theta$, $\pi'$ is a target policy, and $\mathbf{p}^{\pi_\theta}$ and $\mathbf{p}^{\pi'}$ are the feature vectors corresponding to the Behavioral Test functions from $\pi_\theta$ and $\pi'$.  




\subsection{Max-Max Problem: theoretical analysis}



We will analyze our AO algorithm for the Max-Max optimization problem. We show that obtained solutions converge to the local maxima of the objective function. 
Consider the function $F(\theta, \mathbf{p}^{\lambda_{\pi_{\theta}}}, \mathbf{p}^{\lambda_{\pi^{\prime}}})$ as in \ref{equation::theory_objective}. We denote by $(\theta^{*}, \mathbf{p}_{*}^{\lambda_{\pi_{\theta}}}, \mathbf{p}_{*}^{\lambda_{\pi^{\prime}}})$
some of its local maxima. Define $\tilde{F}(\theta) = F(\theta, \mathbf{p}_{*}^{\lambda_{\pi_{\theta}}}, \mathbf{p}_{*}^{\lambda_{\pi^{\prime}}})$, i.e. $\tilde{F}$ is $F$ as a function of $\theta$ for locally optimal values of $\mathbf{p}^{\lambda_{\pi_{\theta}}}$ and $\mathbf{p}^{\lambda_{\pi^{\prime}}}$.


We will assume that $\tilde{F}$ is locally $\zeta$-strongly concave
and $\delta$-smooth for some fixed $\zeta, \delta>0$ in the neighborhood $N(\theta^{*}, r)$ of its optimal value $\theta^{*}$. We will also assume that 
gradient of $\tilde{F}$ is $L_{2}$-Lipschitz with Lipschitz coefficient $\phi$ in that neighborhood. The following convergence theorem holds:

\begin{comment}

\begin{theorem}
\label{maxmaxtheorem}
For the entropy coefficient $\gamma$, denote: $\phi_{\gamma}=\frac{1}{2\gamma}e^{\frac{4}{\gamma}}$, and $u_{\gamma}=\frac{8}{3\gamma}e^{\frac{4}{\gamma}}$.
Denote $\phi_{*} = \max(\phi, \phi_{\gamma})$ and $\xi = \min (\frac{2\delta \zeta}{\delta + \zeta},u_{\gamma})$. Let $s(t)=(\theta(t), \mathbf{p}^{\lambda_{\pi_{\theta}}}(t), \mathbf{p}^{\lambda_{\pi^{\prime}}}(t))$ be the solution from iteration $t$ and $s_{*}$ the local maximum considered above. Assume that optimization starts in $\theta_{0} \in N(\theta^{*},r)$.
If $\phi_{*} < \frac{2\xi}{3}$, then the error at iteration $t+1$ of the presented AO algorithm for the Max-Max problem with decaying gradient step size $\alpha^t = \frac{3/2}{[2\xi-3\phi_{*}](t+2) + \frac{3}{2}\phi_{*}}$ satisfies for $\sigma = \sqrt{2(1+e^{\frac{2}{\gamma}})^{2} + \sup_{N(\theta^{*}),r)}
\nabla_{\theta} \tilde{F}(\theta)^{2}}$:
\begin{equation}
%vspace{-0.1in}
\mathbb{E}[\|s(t+1)-s_{*}\|^{2}_{2}] \leq \mathbb{E}[\|s(0)-s_{*}\|^{2}_{2}](\frac{2}{t+3})^{\frac{3}{2}}
+ \sigma^2\frac{9}{[2\xi-3\phi_{*}]^2(t+3)},
\end{equation}
\end{theorem}
% 

Local concavity is necessary to obtain strict theoretical guarantees for the optimization of blackbox functions and smoothness assumptions are motivated by the fact that most RL algorithms deal with smoothings of the original blackbox functions (see our discussion on ES methods).

%\begin{comment}
Let us reexamine the assumptions we put on $\tilde{F}$. We do not claim that our algorithm converges to the globally optimal, but rather locally optimal policy, thus local concavity assumption is reasonable and in fact necessary for optimization problems involving blackbox functions (in our case:  $\mathcal{L}(\theta)=\mathbb{E}_{\tau \sim \pi_{\theta}}[\mathcal{R}(\tau)]$). Smoothness might seem problematic at first glance for RL blackbox functions involving contact, but note that most RL algorithms deal with smoothings of the original blackbox functions. That is true even for ES-type algorithms that can be reinterpreted as gradient-based optimizers of Gaussian smoothings \cite{stockholm} approximating gradients via MC methods (see: Section \ref{rl}).
\end{comment}
 
 

Our goal in this section is to prove the following Theorem:

\begin{theorem}
\label{maxmaxtheorem_appendix}
For the entropy coefficient $\gamma$, denote: $\phi_{\gamma}=\frac{1}{2\gamma}e^{\frac{4}{\gamma}}$, and $u_{\gamma}=\frac{8}{3\gamma}e^{\frac{4}{\gamma}}$.
Denote $\phi_{*} = \max(\phi, \phi_{\gamma})$ and $\xi = \min (\frac{2\delta \zeta}{\delta + \zeta},u_{\gamma})$. Let $s(t)=(\theta(t), \mathbf{p}^{\lambda_{\pi_{\theta}}}(t), \mathbf{p}^{\lambda_{\pi^{\prime}}}(t))$ be the solution from iteration $t$ and $s_{*}$ the local maximum considered above. Assume that optimization starts in $\theta_{0} \in N(\theta^{*},r)$.
If $\phi_{*} < \frac{2\xi}{3}$, then the error at iteration $t+1$ of the presented AO algorithm for the Max-Max problem with decaying gradient step size $\alpha^t = \frac{3/2}{[2\xi-3\phi_{*}](t+2) + \frac{3}{2}\phi_{*}}$ satisfies:
\vspace{-0.1in}
\begin{equation}
\mathbb{E}[\|s(t+1)-s_{*}\|^{2}_{2}] \leq \mathbb{E}[\|s(0)-s_{*}\|^{2}_{2}](\frac{2}{t+3})^{\frac{3}{2}}
+ \sigma^2\frac{9}{[2\xi-3\phi_{*}]^2(t+3)},
\end{equation}
where $\sigma = \sqrt{2(1+e^{\frac{2}{\gamma}})^{2} + \sup_{N(\theta^{*}),r)}
\nabla_{\theta} \tilde{F}(\theta)^{2}}$. 
\end{theorem}

We will need several auxiliary technical results.
We will use the following notation: $W_{\gamma}(\theta, \beta_{1},\beta_{2}) = F(\theta, \mathbf{p}^{\lambda_{\pi_{\theta}}},\mathbf{p}^{\lambda_{\pi_{\prime}}})$,
where $F$ is the objective function from the main body of the paper parameterised by entropy coefficient $\gamma>0$,
$\beta_{1} = \mathbf{p}^{\lambda_{\pi_{\theta}}}$ and 
$\beta_{2} = \mathbf{p}^{\lambda_{\pi_{\prime}}}$.
We will apply this notation also in the next section regarding the Min-Max Problem.
For completeness, the definitions of strong concavity, smoothness and Lipschitz condition from Theorem \ref{maxmaxtheorem_appendix} are given in Section \ref{sec:assumptions_1}.

We consider the dual optimization problem:

\begin{eqnarray*}
&&\max_{\theta} \max_{\lambda_1 \in \mathcal{C}(\mathcal{X}),\lambda_2 \in \mathcal{C}(\mathcal{Y})}W_{\gamma}(\theta, \beta_1, \beta_2)\\ &&=\max_{\theta} \max_{\lambda_1 \in \mathcal{C}(\mathcal{X}),\lambda_2 \in \mathcal{C}(\mathcal{Y})}\mathbb{E}_{(x,y,\kappa^{x,1},\dots,\kappa^{x,D},\kappa^{y,1},\dots,\kappa^{y,D})\sim \mu \times \nu \times \omega \times \dots \times \omega}\\
&&\hspace{0.35in}\left[\mathcal{L}(\theta) + \lambda_1(\Phi(x)) + \lambda_2(\Phi(y)) - \gamma\exp\left(\frac{\lambda_1(\Phi(x)) + \lambda_2(\Phi(y)) - C(\Phi(x),\Phi(y))}{\gamma}\right)\right],
\end{eqnarray*}
where $\gamma$ is a parameter, $\mu=\pi_{\theta}$, $\nu=\pi^{\prime}$, $\Phi$ is a fixed trajectories' embedding and furthermore:
\begin{eqnarray*}
\lambda_1(z) &=& \beta_1^{\top}f(z)\\
\lambda_2(z) &=& \beta_2^{\top}f(z),
\end{eqnarray*}
such that $f(\cdot)$ is a random feature vector. The $i^{\text{th}}$ entry of the feature vector is constructed as follows: $[f(z)]_i = \sqrt{\frac{2}{D}}\cos(z^{\top}w^{z,i} + b^{z,i})$, where $w^{z,i} \sim \mathbb{N}\left(0,\mathbb{I}_n\frac{1}{\rho^2}\right)$ and $b^{z,i}\sim \text{Uniform}(0,2\pi)$. For the ease of notation we denote $\kappa^{z,i} = (w^{z,i},b^{z,i})\sim \omega$.
We consider stochastic gradient ascent optimization strategy of the following form:
\begin{itemize}
    \item at time $t$ we receive a \textit{single sample} $(x_t,y_t,\kappa^{x_t,1}_t,\dots,\kappa^{x_t,D}_t,\kappa^{y_t,1}_t,\dots,\kappa^{y_t,D}_t)\sim\mu \times \nu\times \omega\times\dots\times\omega$, then we form feature vectors $[f(x_t)]_i = \sqrt{\frac{2}{D}}\cos(x_t^{\top}w_t^{x_t,i} + b_t^{x_t,i})$ and $[f(y_t)]_i = \sqrt{\frac{2}{D}}\cos(y_t^{\top}w_t^{y_t,i} + b_t^{y_t,i})$, and finally update:
    \begin{itemize}
        \item[] 
        $\beta_1^{t+1}\leftarrow \Pi_1\left[\beta_1^{t} + \alpha_t f(x_t)\left(1 - \exp\left(\frac{(\beta_1^t)^{\top}f(x_t) + (\beta_2^t)^{\top}f(y_t) - C(x,y)}{\gamma}\right)\right)\right]$\\
        \item[] $\beta_2^{t+1}\leftarrow \Pi_2\left[\beta_2^{t} + \alpha_t f(y_t)\left(1 - \exp\left(\frac{(\beta_1^{t+1})^{\top}f(x_t) + (\beta_2^t)^{\top}f(y_t) - C(x,y)}{\gamma}\right)\right)\right]$.
    \end{itemize}
\end{itemize}
$\Pi_d$ ($d=1,2$) denotes the projection onto the Euclidean ball $B_2(\frac{r_d}{2},\beta_d^0)$ of some given radius $\frac{r_d}{2}$ centered at the initial iterate $\beta_d^0$. 

Let $\{\beta_1^{*},\beta_2^{*}\}$ denote the global optimum of $W_{\gamma}(\beta_1,\beta_2)$ computed on the entire data population, i.e. given access to an infinite number of samples (``oracle''). Let $B_2(r,\beta)$ denote the Euclidean ball  of radius $r$ centered at $\beta$.
For the sake of the theoretical analysis we assume that  (a lower-bound on) the radii of convergence $r_1,r_2$ for $\beta_1, \beta_2$, respectively, is known to the algorithm (this assumption is potentially easy to eliminate with a more careful choice of the step size in the first iterations). To be more specific, if at any point in time parameter $\beta_1$ or $\beta_2$ falls outside the ball $B_2(r_1,\beta_1^{*})$ or $B_2(r_2,\beta_2^{*})$, respectively, the projection is applied that pushes the parameter of interest to stay in the ball. Also, let $\nabla_{\beta_1}W_{\gamma}^1(\beta_1,\beta_2)$ and $\nabla_{\beta_2}W_{\gamma}^1(\beta_1,\beta_2)$ denote the gradients of $W_{\gamma}$ with respect to ${\beta_1}$ and ${\beta_2}$, respectively, computed for a single sample. Similarly, $\nabla_{\beta_1} W_{\gamma}(\beta_1,\beta_2)$ and $\nabla_{\beta_2} W_{\gamma}(\beta_1,\beta_2)$ be the gradient of $W_{\gamma}$ with respect to ${\beta_1}$ and ${\beta_2}$, respectively, computed for the entire data population, i.e. infinite number of samples.

Note that given any initial vector $\beta_d^{0}$ in the ball of radius $\frac{r_d}{2}$ centered at $\beta_d^{*}$, we are guaranteed that all iterates remain within an $r_d$-ball of $\beta_d^{*}$. This is true for all $d = 1,2$. The projection is necessary for theoretical analysis but in practice makes little difference. The above is a two-step alternated optimization scheme.

 Let the \textit{population gradient operator}, $\mathcal{G}_d(\beta_1,\beta_2)$, where $d = 1,2$, be defined as
\[
\mathcal{G}_d(\beta_1,\beta_2) \coloneqq \beta_d + \alpha\nabla_{\beta_d} W_{\gamma}(\beta_1,\beta_2).
\]

\subsubsection{Assumptions}
\label{sec:assumptions_1}

Let $W^*_{\gamma,1}(\beta_1)=W_{\gamma}(\beta_1,\beta_2^{*})$ and $W^*_{\gamma,2}(\beta_2)=W_{\gamma}(\beta_1^{*},\beta_2)$. Let $\Omega_1,\Omega_2$ denote non-empty compact convex sets such $\beta_1\in\Omega_1$ and $\beta_2\in\Omega_2$. The following assumptions are made: 

\begin{assumption}[{\em Strong concavity}]
For $d = 1,2$, the function $W^*_{\gamma,d}(\beta_d)$ is $\zeta_d$-strongly concave near $\beta_d^{*}$, i.e. for all pairs $(a_d,b_d)$ in the neighborhood of $\beta_d^{*}$ the following holds
\begin{equation*}
W^*_{\gamma,d}(a_d) - W^*_{\gamma,d}(b_d) - \left<\nabla_{\beta_d} W^*_{\gamma,d}(b_d), a_d-b_d\right>
\leq -\frac{\zeta_d}{2}\|a_d - b_d\|^2_2,
\end{equation*}
% \begin{eqnarray}
% &&L(\beta_1^{*},\dots,\beta_{d-1}^{*},\beta_{d,1},\beta_{d+1}^{*},\dots,\beta_K^{*}) - L(\beta_1^{*},\dots,\beta_{d-1}^{*},\beta_{d,2},\beta_{d+1}^{*},\dots,\beta_K^{*})\nonumber\\
% &&- \left<\nabla_{\beta_d} L(\beta_1^{*},\dots,\beta_{d-1}^{*},\beta_{d,2},\beta_{d+1}^{*},\dots,\beta_K^{*}), \beta_{d,1}-\beta_{d,2}\right>\nonumber\\
% &&\leq -\frac{\zeta_d}{2}\|\beta_{d,1} - \beta_{d,2}\|^2_2,\:\:
% \end{eqnarray}
where $\zeta_d > 0$ is the strong concavity modulus. 
\label{def:strongconN}
\end{assumption}

\begin{assumption}[{\em Smoothness}]
For $d = 1,2$, the function $W^*_{\gamma,d}(\beta_d)$ is $\delta_d$-smooth, i.e.  for all pairs $(a_d,b_d)$ the following holds
\begin{equation*}
W^*_{\gamma,d}(a_d) - W^*_{\gamma,d}(b_d) - \left<\nabla_{\beta_d} W^*_{\gamma,d}(b_d), a_d-b_d\right>
\geq -\frac{\delta_d}{2}\|a_d - b_d\|^2_2,
\end{equation*}
% \begin{eqnarray}
% &&L(\beta_1^{*},\dots,\beta_{d-1}^{*},\beta_{d,1},\beta_{d+1}^{*},\dots,\beta_K^{*}) -L(\beta_1^{*},\dots,\beta_{d-1}^{*},\beta_{d,2},\beta_{d+1}^{*},\dots,\beta_K^{*})\nonumber\\
% &&- \left<\nabla_{\beta_d} L(\beta_1^{*},\dots,\beta_{d-1}^{*},\beta_{d,2},\beta_{d+1}^{*},\dots,\beta_K^{*}), \beta_{d,1}-\beta_{d,2}\right>\nonumber\\
% &&\geq -\frac{\delta_d}{2}\|\beta_{d,1} - \beta_{d,2}\|^2_2,
% \end{eqnarray}
where $\delta_d > 0$ is the smoothness constant. \label{def:smoothN}
\end{assumption}

\begin{assumption}[Gradient stability (GS) / Lipschitz condition]
We assume $W_{\gamma}(\beta_1,\beta_2)$ satisfy GS ($\phi_d$) condition, for all $d=1,2$, over Euclidean balls $\beta_1 \in B_2(r_1,\beta_1^{*}),\beta_2 \in B_2(r_{2},\beta_2^{*})$ given as follows
\[ 
\|\nabla_{\beta_d} W^*_{\gamma,d}(\beta_d) -\nabla_{\beta_d} W_{\gamma}(\beta_1, \beta_2)\|_2\leq \phi_d\|\beta_{\bar{d}} - \beta_{\bar{d}}^{*}\|_2,
\]
where $\phi_d > 0$ and $\bar{d} = (d \mod 2)+1$.
% \begin{eqnarray}
% &&\|\nabla_{\beta_d} L(\beta_1^{*},\dots,\beta_{d-1}^{*},\beta_d,\beta_{d+1}^{*},\dots,\beta_K^{*})-\nabla_{\beta_d} L(\beta_1,\dots,\beta_{d-1},\beta_d,\beta_{d+1},\dots,\beta_K)\|_2\nonumber\\
% &&\leq \gamma_d\sum_{\substack{i=1 \\ i\neq d}}^K\|\beta_i - \beta_i^{*}\|_2.
% \end{eqnarray}
\label{def:GSN}
\end{assumption}

Finally, define the bound $\sigma$ that considers the expected value of the norm of gradients of our objective function as follows: $\sigma = \sqrt{\sigma_1^2+\sigma_2^2}$, where $\sigma_{d}^2 = \sup\{\mathbb{E}[\|\nabla_{\beta_d} W_{\gamma}^1(\beta_1,\beta_2)\|_2^2] : \beta_1 \in B_2(r_1,\beta_1^{*}),\beta_2 \in B_2(r_2,\beta_2^{*}) \}$ for $d=1,2$.

\subsubsection{Main theorems}

\begin{theorem}
Given the stochastic gradient iterates of Max-Max method with decaying step size $\{\alpha^t\}_{t=0}^{\infty}$ and with $\phi < \frac{2\xi}{3}$ the error  at iteration $t+1$ satisfies the recursion
\vspace{-0.1in}
\begin{equation}
\mathbb{E}\left[\|\beta_1^{t+1} - \beta_1^{*}\|_2^2+\|\beta_2^{t+1} - \beta_2^{*}\|_2^2\right] \leq (1-q^t)\mathbb{E}\left[\|\beta_1^{t} - \beta_1^{*}\|_2^2+\|\beta_2^{t} - \beta_2^{*}\|_2^2\right] \nonumber + \frac{(\alpha^t)^2}{1-\alpha^t\phi}\sigma^2,
\end{equation}
\vspace{-0.1in}
where $\phi = \max_{d=1,2}(\phi_d)$, $q^t = 1 - \frac{1-2\alpha^t\xi+2\alpha^t\phi}{1-\alpha^t\phi}$, and $\xi = \min_{d=1,2}\left(\frac{2\delta_d\zeta_d}{\delta_d + \zeta_d}\right)$.
\label{thm:erroruN}
\end{theorem}
The recursion in Theorem \ref{thm:erroruN} is expanded yielding the convergence theorem:

\begin{theorem}
\label{convergence_1}
Given the stochastic gradient iterates of Max-Max method with decaying step size $\alpha^t = \frac{3/2}{[2\xi-3\phi](t+2) + \frac{3}{2}\phi}$ and assuming that $\phi < \frac{2\xi}{3}$, the error at iteration $t+1$ satisfies
\vspace{-0.1in}
\begin{equation}
\mathbb{E}\left[\|\beta_1^{t+1} \!-\! \beta_1^{*}\|_2^2+\|\beta_2^{t+1} \!-\! \beta_2^{*}\|_2^2\right] \leq \mathbb{E}\left[\|\beta_1^0 \!-\! \beta_1^{*}\|_2^2+\|\beta_2^0 \!-\! \beta_2^{*}\|_2^2\right]\left(\!\frac{2}{t+3}\!\right)^{\frac{3}{2}}\nonumber\!\!+ \sigma^2\frac{9}{[2\xi-3\phi]^2(t+3)},
\end{equation}
where $\phi = \max_{d=1,2}(\phi_d)$ and $\xi = \min_{d=1,2}\left(\frac{2\delta_d\zeta_d}{\delta_d + \zeta_d}\right)$.
\label{lem:errorfinal}
\end{theorem}

\subsubsection{Analysis}

The theoretical analysis we provide below is an extension of the analysis in~\cite{balakrishnan2017} to the two-step alternated optimization scheme.

Proof of Theorem \ref{lem:errorfinal} relies on Theorem \ref{thm:erroruN}, which in turn relies on Theorem \ref{thm:contractivityG1wideN} and Lemma \ref{lem:contru2N}, both of which are stated below. Proofs of the lemma and theorems follow in the subsequent subsections.

The next result is a standard result from convex optimization (Theorem 2.1.14 in~\cite{Nesterov:2014:ILC:2670022}) and is used in the proof of Theorem~\ref{thm:contractivityG1wideN} below.

\begin{lemma}
The gradient operator $\mathcal{G}_1(\beta_1,\beta_2^{*})$ under Assumption~\ref{def:strongconN} (strong concavity) and Assumption~\ref{def:smoothN} (smoothness) with constant step size choice $0 < \alpha \leq \frac{2}{\delta_1 + \zeta_1}$ is contractive, i.e.
\begin{equation}
\|\mathcal{G}_1(\beta_1,\beta_2^{*}) - \beta_1^{*}\|_2 \leq \left(1 - \frac{2\alpha\delta_1\zeta_1}{\delta_1 + \zeta_1}\right)\|\beta_1 - \beta^{*}_1\|_2
\label{eq:contractivityTN}
\end{equation}
for all $\beta_1 \in B_2(r_1,\beta_1^{*})$.

Similarly, the gradient operator $\mathcal{G}_2(\beta_1^{*},\beta_2)$ under Assumption~\ref{def:strongconN} (strong concavity) and Assumption~\ref{def:smoothN} (smoothness) with constant step size choice $0 < \alpha \leq \frac{2}{\delta_2 + \zeta_2}$ is contractive, i.e.
\begin{equation}
\|\mathcal{G}_2(\beta_1^{*},\beta_2) - \beta_2^{*}\|_2 \leq \left(1 - \frac{2\alpha\delta_2\zeta_2}{\delta_2 + \zeta_2}\right)\|\beta_2 - \beta^{*}_2\|_2
\label{eq:contractivityTN}
\end{equation}
for all $\beta_2 \in B_2(r_2,\beta_2^{*})$.
\label{lem:contru2N}
\end{lemma}

The next theorem also holds for $d=1,2$. Let $r_1, r_2 > 0$ and $\beta_1 \in B_2(r_1,\beta_1^{*}),\beta_{2} \in B_2(r_{2},\beta_{2}^{*})$.

\begin{theorem}
For some radius $r_d > 0$ ($d=1,2$) and a triplet $(\phi_d,\zeta_d,\delta_d)$ such that $0 \leq \phi_d < \zeta_d \leq \delta_d$, suppose that the function $W_{\gamma,d}^{*}(\beta_d)$ is $\zeta_d$-strongly concave and $\delta_d$-smooth, and that the GS ($\phi_d$) condition holds. Then the population gradient operator $\mathcal{G}_d(\beta_1,\beta_2)$ with step $\alpha$ such that $0 < \alpha \leq \min_{d = 1,2}\frac{2}{\delta_d + \zeta_d}$ is contractive over a ball $B_2(r_d,\beta_d^{*})$, i.e.
\begin{equation}
\|\mathcal{G}_d(\beta_1,\beta_2) - \beta_d^{*}\|_2 \leq (1-\xi\alpha)\|\beta_d - \beta_d^{*}\|_2 + \alpha\phi\|\beta_{\bar{d}}-\beta_{\bar{d}}^{*}\|_2
\end{equation}
\vspace{-0.15in}

where $\bar{d} = (d \mod 2) + 1$, $\phi \coloneqq \max_{d=1,2}\phi_d$, and $\xi \coloneqq \min_{d = 1,2}\frac{2\delta_d\zeta_d}{\delta_d + \zeta_d}$. \\
\vspace{0.1in}
\label{thm:contractivityG1wideN}
\end{theorem}

\begin{proof}
\begin{eqnarray*}
&&\hspace{-0.25in}\|\mathcal{G}_d(\beta_1,\beta_2) - \beta_d^{*}\|_2=\|\beta_d + \alpha\nabla_{\beta_d} W_{\gamma}(\beta_1,\beta_2) - \beta_d^{*}\|_2\\
&&\hspace{-0.25in}\text{by the triangle inequality (and with $d \neq \bar{d}$) we further get}\\
&&\hspace{-0.25in}\leq\|\beta_d + \alpha\nabla_{\beta_d} W_{\gamma,d}^{*}(\beta_d) - \beta_d^{*}\|_2 + \alpha\|\nabla_{\beta_d} W_{\gamma}(\beta_1,\beta_2) - \nabla_{\beta_d}W_{\gamma,d}^{*}(\beta_d)\|_2\\
&&\hspace{-0.25in}\text{by the contractivity from Lemma~\ref{lem:contru2N} and GS condition}\\
&&\hspace{-0.25in}\leq \left(1 - \frac{2\alpha\delta_d\zeta_d}{\delta_d + \zeta_d}\right)\|\beta_d - \beta_d^{*}\|_2 + \alpha\phi_d\|\beta_{\bar{d}} - \beta_{\bar{d}}^{*}\|_2.
\end{eqnarray*}

\end{proof}

\textbf{Proof of Theorem~\ref{thm:erroruN}}\\

Let $\beta_d^{t+1} = \Pi_d(\tilde\beta_d^{t+1})$, where $\tilde\beta_1^{t+1} \coloneqq \beta^t_1 + \alpha^t\nabla_{\beta_1} W_{\gamma}^1(\beta_1^{t},\beta_2^{t})$ and $\tilde\beta_2^{t+1} \coloneqq \beta^t_2 + \alpha^t\nabla_{\beta_2} W_{\gamma}^1(\beta_1^{t+1},\beta_2^{t})$, where $\nabla_{\beta_d} W_{\gamma}^1$ is the gradient computed with respect to a single sample, $\tilde\beta_1$ and $\tilde\beta_2$ are the updates prior to the projection onto a ball $B_2(\frac{r_d}{2},\beta_d^0)$. Let $\Delta^{t+1}_d \coloneqq \beta_d^{t+1} - \beta_d^{*}$ and $\tilde\Delta_d^{t+1} \coloneqq \tilde\beta_d^{t+1} - \beta_d^{*}$. Thus
\begin{eqnarray*}
     \|\Delta^{t+1}_d\|_2^2 - \|\Delta^t_d\|_2^2 &\leq& \|\tilde\Delta^{t+1}_d\|_2^2 - \|\Delta^t_d\|_2^2\\
    &=&    \|\tilde\beta^{t+1}_d - \beta_d^{*}\| - \|\beta_d^t - \beta_d^{*}\| \nonumber\\
&=&    \left<\tilde\beta_d^{t+1}  -  \beta_d^t, \tilde\beta_d^{t+1}  +  \beta_d^t  -  2\beta_d^{*}\right>.
\label{eqn:tmp1N}
\end{eqnarray*}
Let $\hat{Q}_1^t \coloneqq \nabla_{\beta_1} W_{\gamma}^1(\beta_1^{t},\beta_2^{t})$ and $\hat{Q}_2^t \coloneqq \nabla_{\beta_2} W_{\gamma}^1(\beta_1^{t+1},\beta_2^{t})$. Then we have that $\tilde\beta_d^{t+1} - \beta_d^t = \alpha^t \hat{Q}_d^t$. We combine it with Equation~\ref{eqn:tmp1N} and obtain:
\begin{eqnarray*}
&&\|\Delta^{t+1}_d\|_2^2 - \|\Delta^t_d\|_2^2\\
&\leq& \left<\alpha^t\hat{Q}_d^t,\alpha^t\hat{Q}_d^t + 2(\beta_d^t - \beta_d^{*})\right>\\
&=& (\alpha^t)^2(\hat{Q}_d^t)^{\top}\hat{Q}_d^t + 2\alpha^t(\hat{Q}_d^t)^{\top}(\beta_d^t - \beta_d^{*})\\
&=& (\alpha^t)^2\|\hat{Q}_d^t\|_2^2 + 2\alpha^t\left<\hat{Q}_d^t,\Delta^t_d\right>.
\end{eqnarray*}

Let $Q_1^t \coloneqq \nabla_{\beta_1} W_{\gamma}(\beta_1^{t},\beta_2^{t})$ and $Q_2^t \coloneqq \nabla_{\beta_2} W_{\gamma}(\beta_1^{t+1},\beta_2^{t})$. By the properties of martingales, i.e. iterated expectations and tower property:
\begin{equation}
\mathbb{E}[\|\Delta^{t+1}_d\|_2^2] \leq \mathbb{E}[\|\Delta^t_d\|_2^2] + (\alpha^t)^2\mathbb{E}[\|\hat{Q}_d^t\|_2^2]+ 2\alpha^t\mathbb{E}[\left<Q_d^t,\Delta^t_d\right>]
\label{eq:edeltauN}
\end{equation}
Let $Q_d^{*} \coloneqq \nabla_{\beta_d} W_{\gamma}(\beta_1^{*},\beta_2^{*})$. By self-consistency, i.e. $\beta_d^{*} = \arg\max_{\beta_d\in\Omega_d}W_{\gamma,d}^{*}(\beta_d)$, and convexity of $\Omega_d$ we have that
\[\left<Q_d^{*},\Delta^t_d\right> = \left<\nabla_{\beta_d} W_{\gamma}(\beta_1^{*},\beta_2^{*}),\Delta^t_d\right> = 0.
\]
Combining this with Equation~\ref{eq:edeltauN} we have 
\begin{eqnarray*}
\mathbb{E}[\|\Delta^{t+1}_d\|_2^2] &\leq& \mathbb{E}[\|\Delta^t_d\|_2^2] + (\alpha^t)^2\mathbb{E}[\|\hat{Q}_d^t\|_2^2]+ 2\alpha^t\mathbb{E}[\left<Q_d^t - Q_d^{*},\Delta^t_d\right>].
\label{eq:edeltau2N}
\end{eqnarray*}

Define $\mathcal{G}^t_d \coloneqq \beta_d^t + \alpha^tQ^t_d$ and $\mathcal{G}_d^{t*} \coloneqq \beta_d^{*} + \alpha^tQ_d^{*}$. Thus
\begin{eqnarray*}
&&\alpha^t\left<Q_d^t - Q_d^{*},\Delta^t_d\right>\\
&=& \left<\mathcal{G}_d^t - \mathcal{G}_d^{t*} - (\beta^t_d - \beta_d^{*}), \beta^t_d - \beta_d^{*}\right>\\
&=& \left<\mathcal{G}_d^t - \mathcal{G}_d^{t*},\beta^t_d - \beta_d^{*}\right> - \|\beta^t_d - \beta_d^{*}\|_2^2\\
&&\hspace{-0.35in}\text{by the fact that $\mathcal{G}_d^{t*} = \beta_d^{*} + \alpha^tQ_d^{*} = \beta_d^{*}$ (since $Q_d^{*} = 0$):}\\
&=& \left<\mathcal{G}_d^t - \beta_d^{*},\beta^t_d - \beta_d^{*}\right> - \|\beta^t_d - \beta_d^{*}\|_2^2\\
&&\hspace{-0.35in}\text{by the contractivity of $\mathcal{G}^t$ from Theorem~\ref{thm:contractivityG1wideN}:}\\
&\leq& \left\{(1-\alpha^t\xi)\|\beta_d^t-\beta_d^{*}\| + \alpha^t\phi\left(\sum_{i=1}^{d-1}\|\beta_i^{t+1}-\beta_i^{*}\|_2\right.\right.\left.\left.+    \sum_{i=d+1}^{2}\|\beta_i^{t}-\beta_i^{*}\|_2\right)\right\}\|\beta^t_d - \beta_d^{*}\|_2 - \|\beta^t_d - \beta_d^{*}\|_2^2\\
&\leq&\left\{ (1 - \alpha^t\xi)\|\Delta_d^t\|_2  +  \alpha^t\phi \left(\sum_{i=1}^{d-1}\|\Delta_i^{t+1}\|_2  +     \sum_{i=d+1}^{2}\|\Delta_i^t\|_2 \right) \right\}\cdot\|\Delta^t_d\|_2  -  \|\Delta^t_d\|_2^2\\
\end{eqnarray*}

Combining this result with Equation~\ref{eq:edeltau2N} gives
\begin{eqnarray*}
\mathbb{E}[\|\Delta^{t+1}_d\|_2^2] &\leq& \mathbb{E}[\|\Delta^t_d\|_2^2] + (\alpha^t)^2\mathbb{E}[\|\hat{Q}_d^t\|_2^2]+ 2\mathbb{E}\left[ \left\{  (1 - \alpha^t\xi)\|\Delta_d^t\|_2 + \alpha^t\phi\left(\sum_{i=1}^{d-1}\|\Delta_i^{t+1}\|_2  +     \sum_{i=d+1}^{2}\|\Delta_i^t\|_2 \right)  \right\}\right.\\
&&\hspace{-0.9in}\left.\cdot\|\Delta^t_d\|_2  -  \|\Delta^t_d\|_2^2\right]\\
&\hspace{-1.7in}\leq&\hspace{-0.9in} \mathbb{E}[\|\Delta^t_d\|_2^2] + (\alpha^t)^2\sigma_{d}^2 +  2\mathbb{E}\left[ \left\{ (1 - \alpha^t\xi)\|\Delta_d^t\|_2  +  \alpha^t\phi\left(\sum_{i=1}^{d-1}\|\Delta_i^{t+1}\|_2  +     \sum_{i=d+1}^{2}\|\Delta_i^t\|_2 \right)  \right\}\right.\\
&&\hspace{-0.9in}\left.\cdot\|\Delta^t_d\|_2  -  \|\Delta^t_d\|_2^2 \right].
\end{eqnarray*}

After re-arranging the terms we obtain
\begin{eqnarray*}
&&\mathbb{E}[\|\Delta^{t+1}_d\|_2^2]
\leq (\alpha^t)^2\sigma_{d}^2 + (1 - 2\alpha^t\xi)\mathbb{E}[\|\Delta^t_d\|_2^2]+ 2\alpha^t\phi\mathbb{E} \left[ \left(\sum_{i=1}^{d-1}\|\Delta_i^{t+1}\|_2  +     \sum_{i=d+1}^{2}\|\Delta_i^t\|_2 \right)  \|\Delta^t_d\|_2 \right]\\
&&\hspace{-0.4in}\text{apply $2ab \leq a^2 + b^2$}:\\
&\leq& (\alpha^t)^2\sigma_{d}^2 + (1-2\alpha^t\xi)\mathbb{E}[\|\Delta^t_d\|_2^2]+ \alpha^t\phi\mathbb{E} \left[\sum_{i=1}^{d-1} \left(\|\Delta_i^{t+1}\|_2^2 +\|\Delta^t_d\|_2^2\right) \right] +  \alpha^t\phi\mathbb{E} \left[\sum_{i=d+1}^{2} \left(\|\Delta_i^{t}\|_2^2 + \|\Delta^t_d\|_2^2\right)  \right]\\
&=& (\alpha^t)^2\sigma_{d}^2 + \mathbb{E}[\|\Delta^t_d\|_2^2]\cdot\left[1 - 2\alpha^t\xi  +  \alpha^t\phi \right] +  \alpha^t\phi\mathbb{E} \left[\sum_{i=1}^{d-1}\|\Delta_i^{t+1}\|_2^2\right]    +  \alpha^t\phi\mathbb{E} \left[\sum_{i=d+1}^{2} \|\Delta_i^{t}\|_2^2\right]\\
\end{eqnarray*}

We obtained
\begin{eqnarray*}
&&\mathbb{E}[\|\Delta^{t+1}_d\|_2^2] \leq (\alpha^t)^2\sigma_{d}^2 + [1-2\alpha^t\xi + \alpha^t\phi]\mathbb{E}[\|\Delta^t_d\|_2^2] + \alpha^t\phi\mathbb{E} \left[\sum_{i=1}^{d-1}\|\Delta_i^{t+1}\|_2^2\right] + \alpha^t\phi\mathbb{E} \left[\sum_{i=d+1}^{2} \|\Delta_i^{t}\|_2^2\right]\\
&&\text{we next re-group the terms as follows}\\
&&\mathbb{E}[\|\Delta^{t+1}_d\|_2^2] - \alpha^t\phi\mathbb{E} \left[\sum_{i=1}^{d-1}\|\Delta_i^{t+1}\|_2^2\right]\leq [1-2\alpha^t\xi + \alpha^t\phi]\mathbb{E}[\|\Delta^t_d\|_2^2]+ \alpha^t\phi\mathbb{E} \left[\sum_{i=d+1}^{2} \|\Delta_i^{t}\|_2^2\right] + (\alpha^t)^2\sigma_{d}^2 \\
&&\text{and then sum over $d$ from $1$ to $2$}\\
&&\mathbb{E}\left[\sum_{d=1}^2\|\Delta^{t+1}_d\|_2^2\right] - \alpha^t\phi\mathbb{E} \left[\sum_{d=1}^2\sum_{i=1}^{d-1}\|\Delta_i^{t+1}\|_2^2\right]\\
&&\leq [1 - 2\alpha^t\xi  +  \alpha^t\phi]\mathbb{E}\left[\sum_{d=1}^2\|\Delta^t_d\|_2^2\right]+ \alpha^t\phi\mathbb{E} \left[\sum_{d=1}^2\sum_{i=d+1}^{2} \|\Delta_i^{t}\|_2^2\right]  +  (\alpha^t)^2 \sum_{d=1}^2 \sigma_{d}^2 \\
\end{eqnarray*}
\\

Let $\sigma = \sqrt{\sigma_{1}^2 + \sigma_{2}^2}$. Also, note that
\begin{eqnarray*}
&&\hspace{-0.3in} \mathbb{E}\left[\sum_{d=1}^2\|\Delta^{t+1}_d\|_2^2\right] - \alpha^t\phi\mathbb{E} \left[\sum_{d=1}^2\|\Delta_d^{t+1}\|_2^2\right]\leq \mathbb{E}\left[\sum_{d=1}^2\|\Delta^{t+1}_d\|_2^2\right] - \alpha^t\phi\mathbb{E} \left[\sum_{d=1}^2\sum_{i=1}^{d-1}\|\Delta_i^{t+1}\|_2^2\right]
\end{eqnarray*}
and
\begin{eqnarray*}
&&\hspace{-0.3in} [1 - 2\alpha^t\xi  +  \alpha^t\phi]\mathbb{E}\left[\sum_{d=1}^2\|\Delta^t_d\|_2^2\right]+ \alpha^t\phi\mathbb{E} \left[\sum_{d=1}^2\sum_{i=d+1}^{2} \|\Delta_i^{t}\|_2^2\right]  +  (\alpha^t)^2\sigma^2 \\
&\leq& [1 - 2\alpha^t\xi  +  \alpha^t\phi]\mathbb{E}\left[\sum_{d=1}^2\|\Delta^t_d\|_2^2\right]+ \alpha^t\phi\mathbb{E} \left[\sum_{d=1}^2 \|\Delta_d^{t}\|_2^2\right]+ (\alpha^t)^2\sigma^2 \\
\end{eqnarray*}

Combining these two facts with our previous results yields:
\begin{eqnarray*}
&&\hspace{-0.3in} [1-\alpha^t\phi]\mathbb{E}\left[\sum_{d=1}^2\|\Delta^{t+1}_d\|_2^2\right]\\
&\hspace{-0.2in}\leq&\hspace{-0.15in} [1 - 2\alpha^t\xi  +  \alpha^t\phi]\mathbb{E}\left[\sum_{d=1}^2\|\Delta^t_d\|_2^2\right]+ \alpha^t\phi\mathbb{E} \left[\sum_{d=1}^2 \|\Delta_d^{t}\|_2^2\right] + (\alpha^t)^2\sigma^2 \\
&\hspace{-0.2in}=&\hspace{-0.15in} [1 - 2\alpha^t\xi  +  2\alpha^t\phi]\mathbb{E}\left[\sum_{d=1}^2\|\Delta^t_d\|_2^2\right]  +  (\alpha^t)^2\sigma^2 \\
\end{eqnarray*}
Thus:
\begin{eqnarray*}
\mathbb{E}\left[\sum_{d=1}^2\|\Delta^{t+1}_d\|_2^2\right] &\hspace{-0.1in}\leq&\hspace{-0.1in} \frac{1 - 2\alpha^t\xi  +  2\alpha^t\phi}{1-\alpha^t\phi}\mathbb{E}\left[\sum_{d=1}^2\|\Delta^t_d\|_2^2\right]\\
&\hspace{-0.1in}+&\hspace{-0.1in} \frac{(\alpha^t)^2}{1 -\alpha^t\phi}\sigma^2.
\end{eqnarray*}
Since $\phi < \frac{2\xi}{3}$, $\frac{1 - 2\alpha^t\xi  +  2\alpha^t\phi}{1-\alpha^t\phi} < 1$.

\textbf{Proof of Theorem~\ref{lem:errorfinal}}\\

To obtain the final theorem we need to expand the recursion from Theorem~\ref{thm:erroruN}. We obtained

\begin{eqnarray*}
&&\mathbb{E}\left[\sum_{d=1}^2\|\Delta^{t+1}_d\|_2^2\right]\\ 
&&\leq \frac{1 - 2\alpha^t[\xi  -  \phi]}{1-\alpha^t\phi}\mathbb{E}\left[\sum_{d=1}^2\|\Delta^t_d\|_2^2\right]+ \frac{(\alpha^t)^2}{1 - \alpha^t\phi}\sigma^2\\
&&= \left(1  -  \frac{\alpha^t[2\xi - 3\phi]}{1 - \alpha^t\phi}\right)\mathbb{E}\left[\sum_{d=1}^2\|\Delta^t_d\|_2^2\right] + \frac{(\alpha^t)^2}{1 - \alpha^t\phi}\sigma^2
\end{eqnarray*}
Recall that we defined $q^t$ in Theorem~\ref{thm:erroruN} as
\[q^t = 1 - \frac{1-2\alpha^t\xi+2\alpha^t\phi}{1-\alpha^t\phi} = \frac{\alpha^t[2\xi - 3\phi]}{1 - \alpha^t\phi}
\]
and denote
\[f^t = \frac{(\alpha^t)^2}{1 - \alpha^t\phi}.
\]

Thus we have
\begin{eqnarray*}
&&\mathbb{E}\left[\sum_{d=1}^2\|\Delta^{t+1}_d\|_2^2\right]\leq      (1-q^t)\mathbb{E}\left[\sum_{d=1}^2\|\Delta^t_d\|_2^2\right]  +  f^t\sigma^2\\
&     \leq&      (1-q^t)\left\{(1-q^{t-1})\mathbb{E}\left[\sum_{d=1}^2\|\Delta^{t-1}_d\|_2^2\right]  +  f^{t-1}\sigma^2\right\}+     f^t\sigma^2\\
&     =&      (1 - q^t)(1 - q^{t-1})\mathbb{E}\left[\sum_{d=1}^2\|\Delta^{t-1}_d\|_2^2\right]  +  (1-q^t)f^{t-1}\sigma^2  +f^t\sigma^2\\
&     \leq&      (1 - q^t)(1 - q^{t-1}) \left\{ (1 - q^{t-2})\mathbb{E} \left[\sum_{d=1}^2 \|\Delta^{t-2}_d\|_2^2\right]   +  f^{t-2}\sigma^2 \right\} + (1-q^t)f^{t-1}\sigma^2  +  f^t\sigma^2\\
&     =&      (1 - q^t)(1 - q^{t-1})(1 - q^{t-2})\mathbb{E}\left[\sum_{d=1}^2\|\Delta^{t-2}_d\|_2^2\right]\\
&&    + (1 - q^t)(1 - q^{t-1})f^{t-2}\sigma^2   +  (1 - q^t)f^{t-1} \sigma^2  +  f^t\sigma^2\\
\end{eqnarray*}

We end-up with the following
\begin{eqnarray*}
\mathbb{E}\left[\sum_{d=1}^2\|\Delta^{t+1}_d\|_2^2\right] &\leq& \mathbb{E}\left[\sum_{d=1}^2\|\Delta^0_d\|_2^2\right]\prod_{i=0}^t(1 - q^i)+ \sigma^2\sum_{i=0}^{t-1}f^i\prod_{j=i+1}^t(1 - q^j)  +  f^t\sigma^2.
\end{eqnarray*}
Set $q^t = \frac{\frac{3}{2}}{t+2}$ and 
\begin{eqnarray*}
\alpha^t &=& \frac{q^t}{2\xi-3\phi + q^t\phi}\\
&=& \frac{\frac{3}{2}}{[2\xi-3\phi](t+2) + \frac{3}{2}\phi}.
\end{eqnarray*}
Denote $A = 2\xi-3\phi$ and $B = \frac{3}{2}\phi$. Thus 
\[\alpha^t = \frac{\frac{3}{2}}{A(t+2)+B}
\]
and
\[f^t = \frac{(\alpha^t)^2}{1-\frac{2}{3}B\alpha^t} = \frac{\frac{9}{4}}{A(t+2)[A(t+2)+B]}.
\]

\begin{eqnarray*}
&&\mathbb{E}\left[\sum_{d=1}^2\|\Delta^{t+1}_d\|_2^2\right]\\ &\leq& \mathbb{E}\left[\sum_{d=1}^2\|\Delta^0_d\|_2^2\right]\prod_{i=0}^t\left(1 - \frac{\frac{3}{2}}{i+2}\right)+ \sigma^2\sum_{i=0}^{t-1}\frac{\frac{9}{4}}{A(i+2)[A(i+2)+B]}\prod_{j=i+1}^t\left(1 - \frac{\frac{3}{2}}{j+2}\right)\\
&&+ \sigma^2\frac{\frac{9}{4}}{A(t+2)[A(t+2)+B]}\\
&=& \mathbb{E}\left[\sum_{d=1}^2\|\Delta^0_d\|_2^2\right]\prod_{i=2}^{t+2}\left(1 - \frac{\frac{3}{2}}{i}\right)+ \sigma^2\sum_{i=2}^{t+1}\frac{\frac{9}{4}}{Ai[Ai+B]}\prod_{j=i+1}^{t+2}\left(1 - \frac{\frac{3}{2}}{j}\right)+ \sigma^2\frac{\frac{9}{4}}{A(t+2)[A(t+2)+B]}
\end{eqnarray*}

Since $A>0$ and $B>0$ thus 
\begin{eqnarray*}
&&\mathbb{E}\left[\sum_{d=1}^2\|\Delta^{t+1}_d\|_2^2\right]\\ &\leq& \mathbb{E}\left[\sum_{d=1}^2\|\Delta^0_d\|_2^2\right]\prod_{i=2}^{t+2}\left(1 - \frac{\frac{3}{2}}{i}\right)+ \sigma^2\sum_{i=2}^{t+1}\frac{\frac{9}{4}}{Ai[Ai+B]}\prod_{j=i+1}^{t+2}\left(1 - \frac{\frac{3}{2}}{j}\right)+ \sigma^2\frac{\frac{9}{4}}{A(t+2)[A(t+2)+B]}\\
&\leq& \mathbb{E}\left[\sum_{d=1}^2\|\Delta^0_d\|_2^2\right]\prod_{i=2}^{t+2}\left(1 - \frac{\frac{3}{2}}{i}\right)+ \sigma^2\sum_{i=2}^{t+1}\frac{\frac{9}{4}}{(Ai)^2}\prod_{j=i+1}^{t+2}\left(1 - \frac{\frac{3}{2}}{j}\right)+ \sigma^2\frac{\frac{9}{4}}{[A(t+2)]^2}
\end{eqnarray*}

We can next use the fact that for any $a \in (1,2)$:
\[\prod_{i=\tau+1}^{t+2}\left(1-\frac{a}{i}\right) \leq \left(\frac{\tau+1}{t+3}\right)^a.
\]
The bound then becomes
\begin{eqnarray*}
&&\mathbb{E}\left[\sum_{d=1}^2\|\Delta^{t+1}_d\|_2^2\right]\\ &     \leq&      \mathbb{E}\left[\sum_{d=1}^2\|\Delta^0_d\|_2^2\right]\prod_{i=2}^{t+2}\left(1 - \frac{\frac{3}{2}}{i}\right)  + \sigma^2\sum_{i=2}^{t+1}\frac{\frac{9}{4}}{(Ai)^2}\prod_{j=i+1}^{t+2}\left(1 - \frac{\frac{3}{2}}{j}\right) + \sigma^2\frac{\frac{9}{4}}{[A(t+2)]^2}\\
&     \leq&      \mathbb{E}\left[\sum_{d=1}^2\|\Delta^0_d\|_2^2\right]\left(\frac{2}{t+3}\right)^{\frac{3}{2}} + \sigma^2\sum_{i=2}^{t+1}\frac{\frac{9}{4}}{(Ai)^2}\left(\frac{i+1}{t+3}\right)^{\frac{3}{2}}  + \sigma^2\frac{\frac{9}{4}}{[A(t+2)]^2}\\
&     =&      \mathbb{E}\left[\sum_{d=1}^2\|\Delta^0_d\|_2^2\right]\left(\frac{2}{t+3}\right)^{\frac{3}{2}} + \sigma^2\sum_{i=2}^{t+2}\frac{\frac{9}{4}}{(Ai)^2}\left(\frac{i+1}{t+3}\right)^{\frac{3}{2}}\\
\end{eqnarray*}

Note that $(i+1)^{\frac{3}{2}}\leq 2i$ for $i=2,3,\dots$, thus
\begin{eqnarray*}
&&\mathbb{E}\left[\sum_{d=1}^2\|\Delta^{t+1}_d\|_2^2\right]\\ &     \leq&      \mathbb{E}\left[\sum_{d=1}^2\|\Delta^0_d\|_2^2\right]\left(\frac{2}{t+3}\right)^{\frac{3}{2}} + \sigma^2\frac{\frac{9}{4}}{A^2(t+3)^{\frac{3}{2}}}\sum_{i=2}^{t+2}\frac{(i+1)^{\frac{3}{2}}}{i^2}\\
&     \leq&      \mathbb{E}\left[\sum_{d=1}^2\|\Delta^0_d\|_2^2\right]\left(\frac{2}{t+3}\right)^{\frac{3}{2}} + \sigma^2\frac{\frac{9}{2}}{A^2(t+3)^{\frac{3}{2}}}\sum_{i=2}^{t+2}\frac{1}{i^\frac{1}{2}}\\
&&          \text{finally note that $\sum_{i=2}^{t+2}\frac{1}{i^{\frac{1}{2}}} \leq \int_{1}^{t+2}\frac{1}{x^\frac{1}{2}}dx \leq 2(t+3)^{\frac{1}{2}}$. Thus}\\
&     \leq&      \mathbb{E}\left[\sum_{d=1}^2\|\Delta^0_d\|_2^2\right]\left(\frac{2}{t+3}\right)^{\frac{3}{2}} + \sigma^2\frac{9}{A^2(t+3)}\\
&&          \text{substituting $A = 2\xi-3\phi$ gives}\\
&     =&      \mathbb{E}\left[\sum_{d=1}^2\|\Delta^0_d\|_2^2\right]\left(\frac{2}{t+3}\right)^{\frac{3}{2}} + \sigma^2\frac{9}{[2\xi-3\phi]^2(t+3)}\\
\end{eqnarray*}

This leads us to the final theorem.

\textbf{Proof of Theorem \ref{maxmaxtheorem_appendix}}

In order to prove Theorem \ref{maxmaxtheorem_appendix} it suffices to apply Theorem \ref{convergence_1} and notice that: 
\begin{itemize}
    \item function $h_{\mathbf{v},C}:\mathbb{R}^{d} \rightarrow \mathbb{R}$ defined as follows: $h_{\mathbf{v},C}(\mathbf{w}) = \mathbf{w}^{\top}\mathbf{v} - Ae^{\frac{\mathbf{w}^{\top}\mathbf{v}}{\lambda}}$ for $A=\gamma e^{-\frac{C}{\gamma}}$
is $\frac{2}{\gamma}e^{\frac{4}{\gamma}}$-smooth, $\frac{2}{\gamma}$-strongly concave and its gradient is Lipschitz with Lipschitz coefficient $\frac{1}{2\gamma}e^{\frac{4}{\gamma}}$ (with respect to $L_{2}$-norm) for $C>0$
and $\mathbf{v}$ satisfying: $|\mathbf{w}^{\top}\mathbf{v}| \leq 1$,
\item $\|\nabla h_{\mathbf{v},C}(\mathbf{v})\|^{2}_{2} \leq 2(1+e^{\frac{2}{\gamma}})^{2}$ under above conditions.
\end{itemize}


\subsection{MinMax Problem: theoretical analysis}
In this section we aim to obtain similar results for Min-Max Problem as for Max-Max problem. We will use the same notation as in the main body of the paper. We prove the following results:

\begin{theorem}
\label{minmaxtheorem_appendix}
Denote $\phi_{*} = \max(\phi,\phi_{\gamma})$ and $\xi = \min (\frac{2\delta \zeta}{\delta + \zeta},u_{\gamma})$, where $\phi_{\gamma}$ and $u_{\gamma}$ are as in Theorem \ref{maxmaxtheorem_appendix}. Let $s(t)=(\theta(t), \mathbf{p}^{\lambda_{\pi_{\theta}}}(t), \mathbf{p}^{\lambda_{\pi^{\prime}}}(t))$ be the solution obtained in iteration $t$ and $s_{*}$ the local optimum. Assume that optimization starts in $\theta_{0} \in N(\theta^{*},r)$.
If $\phi_{*} < \frac{\xi}{3}$, then the error at iteration $t+1$ of the alternating optimization algorithm for the Min-Max problem with decaying gradient step size $\alpha^t = \frac{3/2}{[2\xi-6\phi_{*}](t+2) + 3\phi_{*}}$ satisfies:
\vspace{-0.1in}
\begin{equation}
\mathbb{E}[\|s(t+1)-s_{*}\|^{2}_{2}] \leq \mathbb{E}[\|s(0)-s_{*}\|^{2}_{2}](\frac{2}{t+3})^{\frac{3}{2}}
+ \sigma^2\frac{9}{[2\xi-6\phi_{*}]^2(t+3)},
\end{equation}
where $\sigma = \sqrt{2(1+e^{\frac{2}{\gamma}})^{2} + \sup_{N(\theta^{*}),r)}
\nabla_{\theta} \tilde{F}(\theta)^{2}}$.
\end{theorem}

We use the same technical notation as in the previous section, with the only exception that this time we denote: $W_{\gamma}(\theta, \beta_{1}, \beta_{2}) = - F(\theta, \mathbf{p}^{\lambda_{\pi_{\theta}}},\mathbf{p}^{\lambda_{\pi_{\prime}}})$.
We consider the MinMax problem of the following form

\begin{eqnarray*}
&&\min_{\theta}\max_{\lambda_{1} \in \mathcal{C}(\mathcal{X}),\lambda_{2} \in \mathcal{C}(\mathcal{Y})}W_{\gamma}(\theta, \beta_1, \beta_2)\\
&&=\min_{\theta}\max_{\lambda_{1} \in \mathcal{C}(\mathcal{X}),\lambda_{2} \in \mathcal{C}(\mathcal{Y})}\mathbb{E}_{(x,y,\kappa^{x,1},\dots,\kappa^{x,D},\kappa^{y,1},\dots,\kappa^{y,D})\sim \mu \times \nu \times \omega \times \dots \times \omega}\\
&&\hspace{0.35in}\left[-\mathcal{L}(\theta) + \lambda_1(\Phi(x)) + \lambda_2(\Phi(y)) - \gamma\exp\left(\frac{\lambda_1(\Phi(x)) + \lambda_2(\Phi(y)) - C(\Phi(x),\Phi(y))}{\gamma}\right)\right],
\end{eqnarray*}
where $\gamma$ is a parameter and the remaining notation is analogous to the Max-Max case.

We consider mixed stochastic gradient descent/ascend optimization strategy of the following form:
\begin{itemize}
    \item at time $t$ we receive a \textit{single sample} $(x_t,y_t,\kappa^{x_t,1}_t,\dots,\kappa^{x_t,D}_t,\kappa^{y_t,1}_t,\dots,\kappa^{y_t,D}_t)\sim\pi_{\theta^t} \times \nu\times \omega\times\dots\times\omega$, then we form feature vectors $[f(x_t)]_i = \sqrt{\frac{2}{D}}\cos(x_t^{\top}w_t^{x_t,i} + b_t^{x_t,i})$ and $[f(y_t)]_i = \sqrt{\frac{2}{D}}\cos(y_t^{\top}w_t^{y_t,i} + b_t^{y_t,i})$, and finally update:
    \begin{itemize}
        \item[] 
        $\theta^{t+1} \leftarrow \Pi_1\left[\theta^{t} - \alpha_t\nabla_{\theta = \theta^t}W_{\gamma}(\theta,\beta^t_{1}, \beta^t_{2})\right]$\footnote{later we also use alternative notation for gradient $\nabla_{\theta = \theta^t}W_{\gamma}(\theta,\beta^t_{1}, \beta^t_{2})$ as $\nabla_{\theta}W_{\gamma}(\theta^t,\beta^t_{1}, \beta^t_{2})$}\\
        \item[] 
        $\beta_1^{t+1}\leftarrow \Pi_2\left[\beta_{1}^{t} + \alpha_t f(x_t)\left(1 - \exp\left(\frac{(\beta_{1}^t)^{\top}f(x_t) + (\beta_{2}^t)^{\top}f(y_t) - C(x,y)}{\gamma}\right)\right)\right]$\\
        \item[] $\beta_{2}^{t+1}\leftarrow \Pi_3\left[\beta_{2}^{t} + \alpha_t f(y_t)\left(1 - \exp\left(\frac{(\beta_{1}^{t+1})^{\top}f(x_t) + (\beta_{2}^t)^{\top}f(y_t) - C(x,y)}{\gamma}\right)\right)\right]$.
    \end{itemize}
\end{itemize}

$\Pi_1$ denotes the projection onto the Euclidean ball $B_2(\frac{r_1}{2},\theta^0)$ and $\Pi_d$ ($d=1,2$) denotes the projection onto the Euclidean ball $B_2(\frac{r_1}{2},\beta_d^0)$. 

Let $\{\theta^{*}, \beta_1^{*},\beta_2^{*}\}$ denote the the global optimal solution of the saddle point problem $\min_{\theta}\max_{\beta_1,\beta_2}W_{\gamma}(\theta, \beta_1,\beta_2)$ computed on the entire data population, i.e. given access to an infinite number of samples (``oracle''). As before, we assume that (a lower-bound on) the radii of convergence $r_1, r_2,r_3$ for $\theta, \beta_1, \beta_2$, respectively, is known to the algorithm and thus the projection is applied to control $\theta, \beta_1, \beta_2$ to stay in their respective balls. Also, let $\nabla_{\theta}W_{\gamma}^1(\theta,\beta_1,\beta_2)$, $\nabla_{\beta_1}W_{\gamma}^1(\theta,\beta_1,\beta_2)$ and $\nabla_{\beta_2}W_{\gamma}^1(\theta,\beta_1,\beta_2)$ denote the gradients of $W_{\gamma}$ with respect to $\theta$,${\beta_1}$ and ${\beta_2}$, respectively, computed for a single sample. Similarly, $\nabla_{\theta} W_{\gamma}(\theta,\beta_1,\beta_2)$, $\nabla_{\beta_1} W_{\gamma}(\theta,\beta_1,\beta_2)$ and $\nabla_{\beta_2} W_{\gamma}(\theta,\beta_1,\beta_2)$ be the gradient of $W_{\gamma}$ with respect to $\theta$, ${\beta_1}$ and ${\beta_2}$, respectively, computed for the entire data population, i.e. infinite number of samples.

Note that given any initial vector $\theta^{0}$ in the ball of radius $\frac{r_1}{2}$ centered at $\theta^{*}$, we are guaranteed that all iterates remain within an $r_1$-ball of $\theta^{*}$ and given any initial vector $\beta_d^{0}$ ($d=1,2$) in the ball of radius $\frac{r_d}{2}$ centered at $\beta_d^{*}$, we are guaranteed that all iterates remain within an $r_d$-ball of $\beta_d^{*}$. The projection is necessary for theoretical analysis but in practice makes little difference. The above is a three-step alternated optimization scheme.

 Let the \textit{population gradient operator}, $\mathcal{G}_d(\theta,\beta_1,\beta_2)$, where $d = 1,2,3$, be defined as
\[\mathcal{G}_1(\theta,\beta_1,\beta_2) \coloneqq \theta - \alpha\nabla_{\theta} W_{\gamma}(\theta,\beta_1,\beta_2)
\]
and
\[
\mathcal{G}_d(\theta,\beta_1,\beta_2) \coloneqq \beta_d + \alpha\nabla_{\beta_i} W_{\gamma}(\theta,\beta_1,\beta_2) \:\:\:\text{for}\:d=2,3.
\]

\subsubsection{Assumptions}
\label{sec:assumptions_2}

Let $W^*_{\gamma,1}(\theta)=W_{\gamma}(\theta,\beta_1^{*},\beta_2^{*})$, $W^*_{\gamma,2}(\beta_1)=W_{\gamma}(\theta^{*},\beta_1,\beta_2^{*})$ and $W^*_{\gamma,3}(\beta_2)=W_{\gamma}(\theta^{*},\beta_1^{*},\beta_2)$. Let $\Omega_1,\Omega_2,\Omega_3$ denote non-empty compact convex sets such $\theta \in \Omega_1,\beta_1\in\Omega_2$ and $\beta_2\in\Omega_3$. The following assumptions are made: 

\begin{assumption}[{\em Strong convexity/concavity}]
The function $W^*_{\gamma,1}(\theta)$ is $\zeta_1$-strongly convex near $\theta^{*}$ and the functions $W^*_{\gamma,2}(\beta_1)$ and $W^*_{\gamma,3}(\beta_2)$ are $\zeta_2$- and $\zeta_3$-strongly concave, respectively, near $\beta_1^{*}$ and $\beta_2^{*}$, respectively, where $\zeta_1,\zeta_2,\zeta_3 > 0$. 
\label{def:strongconN2}
\end{assumption}

\begin{assumption}[{\em Smoothness}]
The functions $W^*_{\gamma,1}(\theta), W^*_{\gamma,2}(\beta_1)$, and $W^*_{\gamma,3}(\beta_2)$ are $\delta_1$-,$\delta_2$-, and $\delta_3$-smooth, respectively, where $\delta_1, \delta_2, \delta_3 > 0$ are the smoothness constants. 
\label{def:smoothN2}
\end{assumption}

\begin{assumption}[Gradient stability (GS) / Lipschitz condition]
We assume $W_{\gamma}(\theta,\beta_1,\beta_2)$ satisfy GS ($\phi_d$) condition, for all $d=1,2,3$, over Euclidean balls $\theta \in B_2(r_1,\theta^{*}),\beta_1 \in B_2(r_2,\beta_1^{*}),\beta_2 \in B_2(r_3,\beta_2^{*})$ given as follows
\vspace{-0.07}
\[ 
\|\nabla_{\theta} W^*_{\gamma,1}(\theta) -\nabla_{\theta} W_{\gamma}(\theta,\beta_1, \beta_2)\|_2\leq \phi_1\sum_{d=1}^2\|\beta_{d} - \beta_{d}^{*}\|_2,
\]
and for $d = 1,2$
\[ 
\|\nabla_{\beta_d} W^*_{\gamma,d+1}(\beta_d) -\nabla_{\beta_d} W_{\gamma}(\theta,\beta_1, \beta_2)\|_2\leq \phi_d(\|\theta - \theta^{*}\|_2 + \|\beta_{\bar{d}} - \beta_{\bar{d}}^{*}\|_2),
\]
where $\phi_d > 0$ and $\bar{d} = (d \mod 2)+1$.
% \begin{eqnarray}
% &&\|\nabla_{\beta_d} L(\beta_1^{*},\dots,\beta_{d-1}^{*},\beta_d,\beta_{d+1}^{*},\dots,\beta_K^{*})-\nabla_{\beta_d} L(\beta_1,\dots,\beta_{d-1},\beta_d,\beta_{d+1},\dots,\beta_K)\|_2\nonumber\\
% &&\leq \gamma_d\sum_{\substack{i=1 \\ i\neq d}}^K\|\beta_i - \beta_i^{*}\|_2.
% \end{eqnarray}
\label{def:GSN2}
\end{assumption}

Finally, as before, define the bound $\sigma$ that considers the expected value of the norm of gradients of our objective function as follows: $\sigma = \sqrt{\sigma_1^2+\sigma_2^2+\sigma_3^2}$, where $\sigma_1^2 = \sup\{\mathbb{E}[\|\nabla_{\theta} W_{\gamma}^1(\theta,\beta_1,\beta_2)\|_2^2] : \theta \in B_2(r_1,\theta^{*}),\beta_1 \in B_2(r_2,\beta_1^{*}),\beta_2 \in B_2(r_3,\beta_2^{*}) \}$ and for $d=1,2$ $\sigma_{d+1}^2 = \sup\{\mathbb{E}[\|\nabla_{\beta_d} W_{\gamma}^1(\theta,\beta_1,\beta_2)\|_2^2] : \theta \in B_2(r_1,\theta^{*}),\beta_1 \in B_2(r_2,\beta_1^{*}),\beta_2 \in B_2(r_3,\beta_2^{*}) \}$.

\subsubsection{Main theorems}

\begin{theorem}
Given the stochastic gradient iterates of MinMax method with decaying step size $\{\alpha^t\}_{t=0}^{\infty}$ and with $\phi < \frac{\xi}{3}$ the error  at iteration $t+1$ satisfies the recursion
\begin{eqnarray}
&&\mathbb{E}\left[\|\theta^{t+1} - \theta^{*}\|_2^2 + \|\beta_1^{t+1} - \beta_1^{*}\|_2^2+\|\beta_2^{t+1} - \beta_2^{*}\|_2^2\right] \nonumber\\
&&\hspace{0.3in}\leq (1-q^t)\mathbb{E}\left[\|\theta^{t} - \theta^{*}\|_2^2 + \|\beta_1^{t} - \beta_1^{*}\|_2^2+\|\beta_2^{t} - \beta_2^{*}\|_2^2\right] + \frac{(\alpha^t)^2}{1-2\alpha^t\phi}\sigma^2 \nonumber,
\end{eqnarray}
\vspace{-0.1in}
where $\phi = \max_{d=1,2,3}(\phi_d)$, $q^t = 1 - \frac{1-2\alpha^t\xi+4\alpha^t\phi}{1-2\alpha^t\phi}$, and $\xi = \min_{d=1,2,3}\left(\frac{2\delta_d\zeta_d}{\delta_d + \zeta_d}\right)$.
\label{thm:erroruN2}
\end{theorem}
The recursion in Theorem \ref{thm:erroruN} is expanded yielding the convergence theorem:

\begin{theorem}
\label{convergence_2}
Given the stochastic gradient iterates of MinMax method with decaying step size $\alpha^t = \frac{3/2}{[2\xi-6\phi](t+2) + 3\phi}$ and assuming that $\phi < \frac{\xi}{3}$, the error at iteration $t+1$ satisfies
\begin{eqnarray}
&&\mathbb{E}\left[\|\theta^{t+1} - \theta^{*}\|_2^2 + \|\beta_1^{t+1} - \beta_1^{*}\|_2^2+\|\beta_2^{t+1} - \beta_2^{*}\|_2^2\right] \nonumber\\
&&\hspace{0.3in}\leq\mathbb{E}\left[\|\theta^0 - \theta^{*}\|_2^2 + \|\beta_1^0 - \beta_1^{*}\|_2^2+\|\beta_2^0 - \beta_2^{*}\|_2^2\right]\left(\frac{2}{t+3}\right)^{\frac{3}{2}} + \sigma^2\frac{9}{[2\xi-6\phi]^2(t+3)} \nonumber,
\end{eqnarray}
where $\phi = \max_{d=1,2,3}(\phi_d)$ and $\xi = \min_{d=1,2,3}\left(\frac{2\delta_d\zeta_d}{\delta_d + \zeta_d}\right)$.
\label{lem:errorfinal2}
\end{theorem}

Proof of Theorem \ref{lem:errorfinal2} relies on Theorem \ref{thm:erroruN2}, which in turn relies on Theorem \ref{thm:contractivityG1wideN2} and Lemma \ref{lem:contruN2}, both of which are stated below. Proofs of the lemma and theorems follow in the subsequent subsections.

\subsubsection{Analysis}
The next result is a standard result from convex optimization (Theorem 2.1.14 in~\cite{Nesterov:2014:ILC:2670022}) and is used in the proof of Theorem~\ref{thm:contractivityG1wideN2} below.

\begin{lemma}
The gradient operator $\mathcal{G}_1(\theta,\beta_1^{*},\beta_2^{*})$ under strong convexity and smoothness assumptions with constant step size choice $0 < \alpha \leq \frac{2}{\delta_1 + \zeta_1}$ is contractive, i.e.
\begin{equation*}
\|\mathcal{G}_1(\theta,\beta_1^{*},\beta_2^{*}) - \theta^{*}\|_2 \leq \left(1 - \frac{2\alpha\delta_1\zeta_1}{\delta_1 + \zeta_1}\right)\|\theta - \theta^{*}\|_2
\end{equation*}
for all $\theta \in B_2(r_1,\theta^{*})$.

Similarly, the gradient operator $\mathcal{G}_1(\theta^{*},\beta_1,\beta_2^{*})$ under strong concavity and smoothness assumptions with constant step size choice $0 < \alpha \leq \frac{2}{\delta_2 + \zeta_2}$ is contractive, i.e.
\begin{equation*}
\|\mathcal{G}_1(\theta^{*},\beta_1,\beta_2^{*}) - \beta_1^{*}\|_2 \leq \left(1 - \frac{2\alpha\delta_2\zeta_2}{\delta_2 + \zeta_2}\right)\|\beta_1 - \beta^{*}_1\|_2
\end{equation*}
for all $\beta_1 \in B_2(r_2,\beta_1^{*})$.

And similarly, the gradient operator $\mathcal{G}_2(\theta^{*},\beta_1^{*},\beta_2)$ under strong concavity and smoothness assumptions with constant step size choice $0 < \alpha \leq \frac{2}{\delta_3 + \zeta_3}$ is contractive, i.e.
\begin{equation*}
\|\mathcal{G}_2(\theta^{*},\beta_1^{*},\beta_2) - \beta_2^{*}\|_2 \leq \left(1 - \frac{2\alpha\delta_3\zeta_3}{\delta_3 + \zeta_3}\right)\|\beta_2 - \beta^{*}_2\|_2
\end{equation*}
for all $\beta_2 \in B_2(r_3,\beta_2^{*})$.
\label{lem:contruN2}
\end{lemma}

The next theorem holds for $d=1,2,3$. Let $r_1, r_2, r_3 > 0$ and $\theta \in B_2(r_1,\theta^{*}),\beta_1 \in B_2(r_2,\beta_1^{*}),\beta_{2} \in B_2(r_3,\beta_{2}^{*})$.

\begin{theorem}
For some radius $r_1$ and a triplet $(\phi_1,\zeta_1,\delta_1)$ such that $0 \leq \phi_1 < \zeta_1 \leq \delta_1$, suppose that the function $W_{\gamma,1}^{*}(\theta)$ is $\zeta_1$-strongly convex and $\delta_1$-smooth and that the GS ($\phi_1$) condition holds. Then the population gradient operator $\mathcal{G}_1(\theta,\beta_1,\beta_2)$ with step $\alpha$ such that $0 < \alpha \leq \min_{d = 1,2,3}\frac{2}{\delta_d + \zeta_d}$ is contractive over a ball $B_2(r_1,\theta^{*})$, i.e.
\begin{equation*}
\|\mathcal{G}_1(\theta,\beta_1,\beta_2) - \theta^{*}\|_2 \leq (1-\xi\alpha)\|\theta - \theta^{*}\|_2 + \alpha\phi\sum_{d=1}^2\|\beta_{d}-\beta_{d}^{*}\|_2
\end{equation*}
\vspace{-0.15in}

where $\phi \coloneqq \max_{d=1,2,3}\phi_d$ and $\xi \coloneqq \min_{d = 1,2,3}\frac{2\delta_d\zeta_d}{\delta_d + \zeta_d}$. \\

For some radius $r_d$ ($d=2,3$) and a triplet $(\phi_d,\zeta_d,\delta_d)$ such that $0 \leq \phi_d < \zeta_d \leq \delta_d$, suppose that the function $W_{\gamma,d}^{*}(\beta_{d-1})$ is $\zeta_d$-strongly concave and $\delta_d$-smooth and that the GS ($\phi_d$) condition holds. Then the population gradient operator $\mathcal{G}_d(\theta,\beta_1,\beta_2)$ with step $\alpha$ such that $0 < \alpha \leq \min_{d = 1,2,3}\frac{2}{\delta_d + \zeta_d}$ is contractive over a ball $B_2(r_d,\beta_d^{*})$, i.e.
\begin{equation*}
\|\mathcal{G}_d(\theta,\beta_1,\beta_2) - \beta_d^{*}\|_2 \leq (1-\xi\alpha)\|\beta_d - \beta_d^{*}\|_2 + \alpha\phi(\|\beta_{\bar{d}}-\beta_{\bar{d}}^{*}\|_2 + \|\theta-\theta^{*}\|_2).
\end{equation*}
\vspace{-0.15in}

where $\bar{d} = ((d-1) \mod 2) + 1$, $\phi \coloneqq \max_{d=1,2,3}\phi_d$, and $\xi \coloneqq \min_{d = 1,2,3}\frac{2\delta_d\zeta_d}{\delta_d + \zeta_d}$. \\



\vspace{0.1in}
\label{thm:contractivityG1wideN2}
\end{theorem}

\begin{proof}

\begin{eqnarray*}
&&\hspace{-0.25in}\|\mathcal{G}_1(\theta,\beta_1,\beta_2) - \theta^{*}\|_2=\|\theta - \alpha\nabla_{\theta} W_{\gamma}(\theta,\beta_1,\beta_2) - \theta^{*}\|_2\\
&&\hspace{-0.25in}\text{by the triangle inequality we further get}\\
&&\hspace{-0.25in}\leq\|\theta - \alpha\nabla_{\theta} W_{\gamma,1}^{*} - \theta^{*}\|_2 + \alpha\|\nabla_{\theta} W_{\gamma}(\theta,\beta_1,\beta_2) - \nabla_{\theta}W_{\gamma,1}^{*}\|_2\\
&&\hspace{-0.25in}\text{by the contractivity from Lemma~\ref{lem:contruN2} and GS condition}\\
&&\hspace{-0.25in}\leq \left(1 - \frac{2\alpha\delta_1\zeta_1}{\delta_1 + \zeta_1}\right)\|\theta - \theta^{*}\|_2 + \alpha\phi_1\sum_{d=1}^2\|\beta_{d} - \beta_{d}^{*}\|_2.
\end{eqnarray*}

The proof of the rest of the theorem is analogous to the proof of Theorem~\ref{thm:contractivityG1wideN}.

\end{proof}

\textbf{Proof of Theorem~\ref{thm:erroruN2}}\\

Let $\theta_1 = \theta$, $\theta_2 = \beta_1$, and $\theta_3 = \beta_2$.

Let $\theta_d^{t+1} = \Pi_d(\tilde\theta_d^{t+1})$, where $\tilde\theta_1^{t+1} \coloneqq \theta^t_1 - \alpha^t\nabla_{\theta_1} W_{\gamma}^1(\theta_1^{t},\theta_2^{t},\theta_3^{t})$, $\tilde\theta_2^{t+1} \coloneqq \theta^t_2 + \alpha^t\nabla_{\theta_2} W_{\gamma}^1(\theta_1^{t+1},\theta_2^{t},\theta_3^{t})$, and $\tilde\theta_3^{t+1} \coloneqq \theta^t_3 + \alpha^t\nabla_{\theta_3} W_{\gamma}^1(\theta_1^{t+1},\theta_2^{t+1},\theta_3^{t})$, where $\nabla_{\theta_d} W_{\gamma}^1$ is the gradient computed with respect to a single sample, $\tilde\theta_1$, $\tilde\theta_2$, and $\tilde\theta_3$ are the updates prior to the projection. Let $\Delta^{t+1}_1 \coloneqq -\theta_1^{t+1} + \theta_1^{*}$ and for $d=2,3$, $\tilde\Delta_d^{t+1} \coloneqq \tilde\theta_d^{t+1} - \theta_d^{*}$. Thus
\begin{eqnarray*}
     \|\Delta^{t+1}_d\|_2^2 - \|\Delta^t_d\|_2^2 &\leq& \|\tilde\Delta^{t+1}_d\|_2^2 - \|\Delta^t_d\|_2^2\\
    &=&    \|\tilde\theta^{t+1}_d - \theta_d^{*}\| - \|\theta_d^t - \theta_d^{*}\| \nonumber\\
&=&    \left<\tilde\theta_d^{t+1}  -  \theta_d^t, \tilde\theta_d^{t+1}  +  \theta_d^t  -  2\theta_d^{*}\right>.
\label{eqn:tmp1N}
\end{eqnarray*}
Let $\hat{Q}_1^t \coloneqq \nabla_{\theta_1} W_{\gamma}^1(\theta_1^{t},\theta_2^{t},\theta_3^{t})$, $\hat{Q}_2^t \coloneqq \nabla_{\theta_2} W_{\gamma}^1(\theta_1^{t+1},\theta_2^{t},\theta_3^{t})$, and $\hat{Q}_3^t \coloneqq \nabla_{\theta_3} W_{\gamma}^1(\theta_1^{t+1},\theta_2^{t+1},\theta_3^t)$. Thus:
\begin{eqnarray*}
&&\|\Delta^{t+1}_d\|_2^2 - \|\Delta^t_d\|_2^2\\
&\leq& \left<\alpha^t\hat{Q}_d^t,\alpha^t\hat{Q}_d^t + 2(\theta_d^t - \theta_d^{*})\right>\\
&=& (\alpha^t)^2(\hat{Q}_d^t)^{\top}\hat{Q}_d^t + 2\alpha^t(\hat{Q}_d^t)^{\top}(\theta_d^t - \theta_d^{*})\\
&=& (\alpha^t)^2\|\hat{Q}_d^t\|_2^2 + 2\alpha^t\left<\hat{Q}_d^t,\Delta^t_d\right>.
\end{eqnarray*}

Let $Q_1^t \coloneqq \nabla_{\theta_1} W_{\gamma}(\theta_1^{t},\theta_2^{t},\theta_3^{t})$, $Q_2^t \coloneqq \nabla_{\theta_2} W_{\gamma}(\theta_1^{t+1},\theta_2^{t},\theta_3^{t})$, and $Q_3^t \coloneqq \nabla_{\theta_3} W_{\gamma}(\theta_1^{t+1},\theta_2^{t+1},\theta_3^{t})$. By the properties of martingales, i.e. iterated expectations and tower property:
\begin{eqnarray*}
\mathbb{E}[\|\Delta^{t+1}_d\|_2^2] &\leq& \mathbb{E}[\|\Delta^t_d\|_2^2] + (\alpha^t)^2\mathbb{E}[\|\hat{Q}_d^t\|_2^2]+ 2\alpha^t\mathbb{E}[\left<Q_d^t,\Delta^t_d\right>]
\end{eqnarray*}
Let $Q_d^{*} \coloneqq \nabla_{\theta_d} W_{\gamma}(\theta_1^{*},\theta_2^{*},\theta_3^{*})$. By self-consistency, i.e. $\theta_d^{*} = \arg\max_{\theta_d\in\Omega_d}W_{\gamma,d}^{*}(\theta_d)$, and convexity of $\Omega_d$ we have that
\[\left<Q_d^{*},\Delta^t_d\right> = \left<\nabla_{\theta_d} W_{\gamma}(\theta_1^{*},\theta_2^{*},\theta_3^{*}),\Delta^t_d\right> = 0.
\]
Combining this with the above inequality yields
\begin{eqnarray*}
\mathbb{E}[\|\Delta^{t+1}_d\|_2^2] &\leq& \mathbb{E}[\|\Delta^t_d\|_2^2] + (\alpha^t)^2\mathbb{E}[\|\hat{Q}_d^t\|_2^2]+ 2\alpha^t\mathbb{E}[\left<Q_d^t - Q_d^{*},\Delta^t_d\right>].
\end{eqnarray*}

Define $\mathcal{G}^t_1 \coloneqq \theta_1^t - \alpha^tQ^t_1$ and $\mathcal{G}_1^{t*} \coloneqq \theta_1^{*} - \alpha^tQ_1^{*}$. Also, for $d=2,3$ define $\mathcal{G}^t_d \coloneqq \theta_d^t + \alpha^tQ^t_d$ and $\mathcal{G}_d^{t*} \coloneqq \theta_d^{*} + \alpha^tQ_d^{*}$. Thus
\begin{eqnarray*}
&&\alpha^t\left<Q_d^t - Q_d^{*},\Delta^t_d\right>\\
&=& \left<\mathcal{G}_d^t - \mathcal{G}_d^{t*} - (\theta^t_d - \theta_d^{*}), \theta^t_d - \theta_d^{*}\right>\\
&=& \left<\mathcal{G}_d^t - \mathcal{G}_d^{t*},\theta^t_d - \theta_d^{*}\right> - \|\theta^t_d - \theta_d^{*}\|_2^2\\
&&\hspace{-0.35in}\text{by the fact that $\mathcal{G}_d^{t*} = \theta_d^{*} + \alpha^tQ_d^{*} = \theta_d^{*}$ (since $Q_d^{*} = 0$):}\\
&=& \left<\mathcal{G}_d^t - \theta_d^{*},\theta^t_d - \theta_d^{*}\right> - \|\theta^t_d - \theta_d^{*}\|_2^2\\
&&\hspace{-0.35in}\text{by the contractivity of $\mathcal{G}^t$ from Theorem~\ref{thm:contractivityG1wideN}:}\\
&\leq& \left\{(1-\alpha^t\xi)\|\theta_d^t-\theta_d^{*}\| + \alpha^t\phi\left(\sum_{i=1}^{d-1}\|\theta_i^{t+1}-\theta_i^{*}\|_2\right.\right.\left.\left.+    \sum_{i=d+1}^{3}\|\theta_i^{t}-\theta_i^{*}\|_2\right)\right\}\|\theta^t_d - \theta_d^{*}\|_2 - \|\theta^t_d - \theta_d^{*}\|_2^2\\
&\leq&\left\{ (1 - \alpha^t\xi)\|\Delta_d^t\|_2  +  \alpha^t\phi \left(\sum_{i=1}^{d-1}\|\Delta_i^{t+1}\|_2  +     \sum_{i=d+1}^{3}\|\Delta_i^t\|_2 \right) \right\}\cdot\|\Delta^t_d\|_2  -  \|\Delta^t_d\|_2^2\\
\end{eqnarray*}

Thus
\begin{eqnarray*}
\mathbb{E}[\|\Delta^{t+1}_d\|_2^2] &\leq& \mathbb{E}[\|\Delta^t_d\|_2^2] + (\alpha^t)^2\mathbb{E}[\|\hat{Q}_d^t\|_2^2]+ 2\alpha^t\mathbb{E}[\left<Q_d^t - Q_d^{*},\Delta^t_d\right>]\\
 &=& \mathbb{E}[\|\Delta^t_d\|_2^2] + (\alpha^t)^2\mathbb{E}[\|\hat{Q}_d^t\|_2^2]+ 2\mathbb{E}\left[ \left\{  (1 - \alpha^t\xi)\|\Delta_d^t\|_2 + \alpha^t\phi\left(\sum_{i=1}^{d-1}\|\Delta_i^{t+1}\|_2  +     \sum_{i=d+1}^{3}\|\Delta_i^t\|_2 \right)  \right\}\right.\\
&&\hspace{2.5in}\left.\cdot\|\Delta^t_d\|_2  -  \|\Delta^t_d\|_2^2\right]\\
&\leq&\mathbb{E}[\|\Delta^t_d\|_2^2] + (\alpha^t)^2\sigma_{d}^2 +  2\mathbb{E}\left[ \left\{ (1 - \alpha^t\xi)\|\Delta_d^t\|_2  +  \alpha^t\phi\left(\sum_{i=1}^{d-1}\|\Delta_i^{t+1}\|_2  +     \sum_{i=d+1}^{3}\|\Delta_i^t\|_2 \right)  \right\}\right.\\
&&\hspace{2.5in}\left.\cdot\|\Delta^t_d\|_2  -  \|\Delta^t_d\|_2^2 \right].
\end{eqnarray*}

After re-arranging the terms we obtain
\begin{eqnarray*}
&&\mathbb{E}[\|\Delta^{t+1}_d\|_2^2]
\leq (\alpha^t)^2\sigma_{d}^2 + (1 - 2\alpha^t\xi)\mathbb{E}[\|\Delta^t_d\|_2^2]+ 2\alpha^t\phi\mathbb{E} \left[ \left(\sum_{i=1}^{d-1}\|\Delta_i^{t+1}\|_2  +     \sum_{i=d+1}^{3}\|\Delta_i^t\|_2 \right)  \|\Delta^t_d\|_2 \right]\\
&&\hspace{-0.4in}\text{apply $2ab \leq a^2 + b^2$}:\\
&\leq& (\alpha^t)^2\sigma_{d}^2 + (1-2\alpha^t\xi)\mathbb{E}[\|\Delta^t_d\|_2^2]+ \alpha^t\phi\mathbb{E} \left[\sum_{i=1}^{d-1} \left(\|\Delta_i^{t+1}\|_2^2 +\|\Delta^t_d\|_2^2\right) \right] +  \alpha^t\phi\mathbb{E} \left[\sum_{i=d+1}^{3} \left(\|\Delta_i^{t}\|_2^2 + \|\Delta^t_d\|_2^2\right)  \right]\\
&=& (\alpha^t)^2\sigma_{d}^2 + \mathbb{E}[\|\Delta^t_d\|_2^2]\cdot\left[1 - 2\alpha^t\xi  +  2\alpha^t\phi \right] +  \alpha^t\phi\mathbb{E} \left[\sum_{i=1}^{d-1}\|\Delta_i^{t+1}\|_2^2\right]    +  \alpha^t\phi\mathbb{E} \left[\sum_{i=d+1}^{3} \|\Delta_i^{t}\|_2^2\right]\\
\end{eqnarray*}

We obtained
\begin{eqnarray*}
&&\mathbb{E}[\|\Delta^{t+1}_d\|_2^2] \leq (\alpha^t)^2\sigma_{d}^2 + [1-2\alpha^t\xi + 2\alpha^t\phi]\mathbb{E}[\|\Delta^t_d\|_2^2] + \alpha^t\phi\mathbb{E} \left[\sum_{i=1}^{d-1}\|\Delta_i^{t+1}\|_2^2\right] + \alpha^t\phi\mathbb{E} \left[\sum_{i=d+1}^{3} \|\Delta_i^{t}\|_2^2\right]\\
&&\text{we next re-group the terms as follows}\\
&&\mathbb{E}[\|\Delta^{t+1}_d\|_2^2] - \alpha^t\phi\mathbb{E} \left[\sum_{i=1}^{d-1}\|\Delta_i^{t+1}\|_2^2\right]\leq [1-2\alpha^t\xi + 2\alpha^t\phi]\mathbb{E}[\|\Delta^t_d\|_2^2]+ \alpha^t\phi\mathbb{E} \left[\sum_{i=d+1}^{3} \|\Delta_i^{t}\|_2^2\right] + (\alpha^t)^2\sigma_{d}^2 \\
&&\text{and then sum over $d$ from $1$ to $3$}\\
&&\mathbb{E}\left[\sum_{d=1}^3\|\Delta^{t+1}_d\|_2^2\right] - \alpha^t\phi\mathbb{E} \left[\sum_{d=1}^3\sum_{i=1}^{d-1}\|\Delta_i^{t+1}\|_2^2\right]\\
&&\leq [1 - 2\alpha^t\xi  +  2\alpha^t\phi]\mathbb{E}\left[\sum_{d=1}^3\|\Delta^t_d\|_2^2\right]+ \alpha^t\phi\mathbb{E} \left[\sum_{d=1}^3\sum_{i=d+1}^{3} \|\Delta_i^{t}\|_2^2\right]  +  2(\alpha^t)^2 \sum_{d=1}^3 \sigma_{d}^2 \\
\end{eqnarray*}
\\

Note that
\begin{eqnarray*}
&&\hspace{-0.3in} \mathbb{E}\left[\sum_{d=1}^3\|\Delta^{t+1}_d\|_2^2\right] - 2\alpha^t\phi\mathbb{E} \left[\sum_{d=1}^3\|\Delta_d^{t+1}\|_2^2\right]\leq \mathbb{E}\left[\sum_{d=1}^3\|\Delta^{t+1}_d\|_2^2\right] - \alpha^t\phi\mathbb{E} \left[\sum_{d=1}^3\sum_{i=1}^{d-1}\|\Delta_i^{t+1}\|_2^2\right]
\end{eqnarray*}
and
\begin{eqnarray*}
&&\hspace{-0.3in} [1 - 2\alpha^t\xi  +  2\alpha^t\phi]\mathbb{E}\left[\sum_{d=1}^3\|\Delta^t_d\|_2^2\right]+ \alpha^t\phi\mathbb{E} \left[\sum_{d=1}^3\sum_{i=d+1}^{3} \|\Delta_i^{t}\|_2^2\right]  +  (\alpha^t)^2\sigma^2 \\
&\leq& [1 - 2\alpha^t\xi  +  2\alpha^t\phi]\mathbb{E}\left[\sum_{d=1}^3\|\Delta^t_d\|_2^2\right]+ 2\alpha^t\phi\mathbb{E} \left[\sum_{d=1}^3 \|\Delta_d^{t}\|_2^2\right]+ (\alpha^t)^2\sigma^2 \\
\end{eqnarray*}

Combining these two facts with our previous results yields:
\begin{eqnarray*}
&&\hspace{-0.3in} [1-2\alpha^t\phi]\mathbb{E}\left[\sum_{d=1}^3\|\Delta^{t+1}_d\|_2^2\right]\\
&\hspace{-0.2in}\leq&\hspace{-0.15in} [1 - 2\alpha^t\xi  +  2\alpha^t\phi]\mathbb{E}\left[\sum_{d=1}^3\|\Delta^t_d\|_2^2\right]+ 2\alpha^t\phi\mathbb{E} \left[\sum_{d=1}^3 \|\Delta_d^{t}\|_2^2\right] + (\alpha^t)^2\sigma^2 \\
&\hspace{-0.2in}=&\hspace{-0.15in} [1 - 2\alpha^t\xi  +  2\alpha^t\phi]\mathbb{E}\left[\sum_{d=1}^3\|\Delta^t_d\|_2^2\right]  +  (\alpha^t)^2\sigma^2 \\
\end{eqnarray*}
Thus:
\begin{eqnarray*}
\mathbb{E}\left[\sum_{d=1}^3\|\Delta^{t+1}_d\|_2^2\right] &\hspace{-0.1in}\leq&\hspace{-0.1in} \frac{1 - 2\alpha^t\xi  +  4\alpha^t\phi}{1-2\alpha^t\phi}\mathbb{E}\left[\sum_{d=1}^3\|\Delta^t_d\|_2^2\right]\\
&\hspace{-0.1in}+&\hspace{-0.1in} \frac{(\alpha^t)^2}{1 -2\alpha^t\phi}\sigma^2.
\end{eqnarray*}
Since $\phi < \frac{\xi}{3}$, $\frac{1 - 2\alpha^t\xi  +  4\alpha^t\phi}{1-2\alpha^t\phi} < 1$.

\textbf{Proof of Theorem~\ref{lem:errorfinal2}}\\

To obtain the final theorem we need to expand the recursion from Theorem~\ref{thm:erroruN}. We obtained

\begin{eqnarray*}
&&\mathbb{E}\left[\sum_{d=1}^3\|\Delta^{t+1}_d\|_2^2\right]\\ 
&&\leq \frac{1 - 2\alpha^t[\xi  -  2\phi]}{1-2\alpha^t\phi}\mathbb{E}\left[\sum_{d=1}^3\|\Delta^t_d\|_2^2\right]+ \frac{(\alpha^t)^2}{1 - 2\alpha^t\phi}\sigma^2\\
&&= \left(1  -  \frac{\alpha^t[2\xi - 6\phi]}{1 - 2\alpha^t\phi}\right)\mathbb{E}\left[\sum_{d=1}^3\|\Delta^t_d\|_2^2\right] + \frac{(\alpha^t)^2}{1 - 2\alpha^t\phi}\sigma^2
\end{eqnarray*}
Recall that we defined $q^t$ in Theorem~\ref{thm:erroruN} as
\[q^t = 1 - \frac{1-2\alpha^t\xi+4\alpha^t\phi}{1-2\alpha^t\phi} = \frac{\alpha^t[2\xi - 6\phi]}{1 - 2\alpha^t\phi}
\]
and denote
\[f^t = \frac{(\alpha^t)^2}{1 - 2\alpha^t\phi}.
\]

Thus we have
\begin{eqnarray*}
&&\mathbb{E}\left[\sum_{d=1}^3\|\Delta^{t+1}_d\|_2^2\right]\leq      (1-q^t)\mathbb{E}\left[\sum_{d=1}^3\|\Delta^t_d\|_2^2\right]  +  f^t\sigma^2\\
&     \leq&      (1-q^t)\left\{(1-q^{t-1})\mathbb{E}\left[\sum_{d=1}^3\|\Delta^{t-1}_d\|_2^2\right]  +  f^{t-1}\sigma^2\right\}+     f^t\sigma^2\\
&     =&      (1 - q^t)(1 - q^{t-1})\mathbb{E}\left[\sum_{d=1}^3\|\Delta^{t-1}_d\|_2^2\right]  +  (1-q^t)f^{t-1}\sigma^2  +f^t\sigma^2\\
&     \leq&      (1 - q^t)(1 - q^{t-1}) \left\{ (1 - q^{t-2})\mathbb{E} \left[\sum_{d=1}^3 \|\Delta^{t-2}_d\|_2^2\right]   +  f^{t-2}\sigma^2 \right\} + (1-q^t)f^{t-1}\sigma^2  +  f^t\sigma^2\\
&     =&      (1 - q^t)(1 - q^{t-1})(1 - q^{t-2})\mathbb{E}\left[\sum_{d=1}^3\|\Delta^{t-2}_d\|_2^2\right]\\
&&    + (1 - q^t)(1 - q^{t-1})f^{t-2}\sigma^2   +  (1 - q^t)f^{t-1} \sigma^2  +  f^t\sigma^2\\
\end{eqnarray*}

We end-up with the following
\begin{eqnarray*}
\mathbb{E}\left[\sum_{d=1}^3\|\Delta^{t+1}_d\|_2^2\right] &\leq& \mathbb{E}\left[\sum_{d=1}^3\|\Delta^0_d\|_2^2\right]\prod_{i=0}^t(1 - q^i)+ \sigma^2\sum_{i=0}^{t-1}f^i\prod_{j=i+1}^t(1 - q^j)  +  f^t\sigma^2.
\end{eqnarray*}
Set $q^t = \frac{\frac{3}{2}}{t+2}$ and 
\begin{eqnarray*}
\alpha^t &=& \frac{q^t}{2\xi-6\phi + 2q^t\phi}\\
&=& \frac{\frac{3}{2}}{[2\xi-6\phi](t+2) + 3\phi}.
\end{eqnarray*}
Denote $A = 2\xi-6\phi$ and $B = 3\phi$. Thus 
\[\alpha^t = \frac{\frac{3}{2}}{A(t+2)+B}
\]
and
\[f^t = \frac{(\alpha^t)^2}{1-\frac{2}{3}B\alpha^t} = \frac{\frac{9}{4}}{A(t+2)[A(t+2)+B]}.
\]

\begin{eqnarray*}
&&\mathbb{E}\left[\sum_{d=1}^2\|\Delta^{t+1}_d\|_2^2\right]\\ &\leq& \mathbb{E}\left[\sum_{d=1}^2\|\Delta^0_d\|_2^2\right]\prod_{i=0}^t\left(1 - \frac{\frac{3}{2}}{i+2}\right)+ \sigma^2\sum_{i=0}^{t-1}\frac{\frac{9}{4}}{A(i+2)[A(i+2)+B]}\prod_{j=i+1}^t\left(1 - \frac{\frac{3}{2}}{j+2}\right)\\
&&+ \sigma^2\frac{\frac{9}{4}}{A(t+2)[A(t+2)+B]}\\
&=& \mathbb{E}\left[\sum_{d=1}^2\|\Delta^0_d\|_2^2\right]\prod_{i=2}^{t+2}\left(1 - \frac{\frac{3}{2}}{i}\right)+ \sigma^2\sum_{i=2}^{t+1}\frac{\frac{9}{4}}{Ai[Ai+B]}\prod_{j=i+1}^{t+2}\left(1 - \frac{\frac{3}{2}}{j}\right)+ \sigma^2\frac{\frac{9}{4}}{A(t+2)[A(t+2)+B]}
\end{eqnarray*}

Since $A>0$ and $B>0$ thus 
\begin{eqnarray*}
&&\mathbb{E}\left[\sum_{d=1}^3\|\Delta^{t+1}_d\|_2^2\right]\\ &\leq& \mathbb{E}\left[\sum_{d=1}^3\|\Delta^0_d\|_2^2\right]\prod_{i=2}^{t+2}\left(1 - \frac{\frac{3}{2}}{i}\right)+ \sigma^2\sum_{i=2}^{t+1}\frac{\frac{9}{4}}{Ai[Ai+B]}\prod_{j=i+1}^{t+2}\left(1 - \frac{\frac{3}{2}}{j}\right)+ \sigma^2\frac{\frac{9}{4}}{A(t+2)[A(t+2)+B]}\\
&\leq& \mathbb{E}\left[\sum_{d=1}^3\|\Delta^0_d\|_2^2\right]\prod_{i=2}^{t+2}\left(1 - \frac{\frac{3}{2}}{i}\right)+ \sigma^2\sum_{i=2}^{t+1}\frac{\frac{9}{4}}{(Ai)^2}\prod_{j=i+1}^{t+2}\left(1 - \frac{\frac{3}{2}}{j}\right)+ \sigma^2\frac{\frac{9}{4}}{[A(t+2)]^2}
\end{eqnarray*}

We can next use the fact that for any $a \in (1,2)$:
\[\prod_{i=\tau+1}^{t+2}\left(1-\frac{a}{i}\right) \leq \left(\frac{\tau+1}{t+3}\right)^a.
\]
The bound then becomes
\begin{eqnarray*}
&&\mathbb{E}\left[\sum_{d=1}^3\|\Delta^{t+1}_d\|_2^2\right]\\ &     \leq&      \mathbb{E}\left[\sum_{d=1}^3\|\Delta^0_d\|_2^2\right]\prod_{i=2}^{t+2}\left(1 - \frac{\frac{3}{2}}{i}\right)  + \sigma^2\sum_{i=2}^{t+1}\frac{\frac{9}{4}}{(Ai)^2}\prod_{j=i+1}^{t+2}\left(1 - \frac{\frac{3}{2}}{j}\right) + \sigma^2\frac{\frac{9}{4}}{[A(t+2)]^2}\\
&     \leq&      \mathbb{E}\left[\sum_{d=1}^3\|\Delta^0_d\|_2^2\right]\left(\frac{2}{t+3}\right)^{\frac{3}{2}} + \sigma^2\sum_{i=2}^{t+1}\frac{\frac{9}{4}}{(Ai)^2}\left(\frac{i+1}{t+3}\right)^{\frac{3}{2}}  + \sigma^2\frac{\frac{9}{4}}{[A(t+2)]^2}\\
&     =&      \mathbb{E}\left[\sum_{d=1}^3\|\Delta^0_d\|_2^2\right]\left(\frac{2}{t+3}\right)^{\frac{3}{2}} + \sigma^2\sum_{i=2}^{t+2}\frac{\frac{9}{4}}{(Ai)^2}\left(\frac{i+1}{t+3}\right)^{\frac{3}{2}}\\
\end{eqnarray*}

Note that $(i+1)^{\frac{3}{2}}\leq 2i$ for $i=2,3,\dots$, thus
\begin{eqnarray*}
&&\mathbb{E}\left[\sum_{d=1}^3\|\Delta^{t+1}_d\|_2^2\right]\\ &     \leq&      \mathbb{E}\left[\sum_{d=1}^2\|\Delta^0_d\|_2^2\right]\left(\frac{2}{t+3}\right)^{\frac{3}{2}} + \sigma^2\frac{\frac{9}{4}}{A^2(t+3)^{\frac{3}{2}}}\sum_{i=2}^{t+2}\frac{(i+1)^{\frac{3}{2}}}{i^2}\\
&     \leq&      \mathbb{E}\left[\sum_{d=1}^3\|\Delta^0_d\|_2^2\right]\left(\frac{2}{t+3}\right)^{\frac{3}{2}} + \sigma^2\frac{\frac{9}{2}}{A^2(t+3)^{\frac{3}{2}}}\sum_{i=2}^{t+2}\frac{1}{i^\frac{1}{2}}\\
&&          \text{finally note that $\sum_{i=2}^{t+2}\frac{1}{i^{\frac{1}{2}}} \leq \int_{1}^{t+2}\frac{1}{x^\frac{1}{2}}dx \leq 2(t+3)^{\frac{1}{2}}$. Thus}\\
&     \leq&      \mathbb{E}\left[\sum_{d=1}^3\|\Delta^0_d\|_2^2\right]\left(\frac{2}{t+3}\right)^{\frac{3}{2}} + \sigma^2\frac{9}{A^2(t+3)}\\
&&          \text{substituting $A = 2\xi-6\phi$ gives}\\
&     =&      \mathbb{E}\left[\sum_{d=1}^3\|\Delta^0_d\|_2^2\right]\left(\frac{2}{t+3}\right)^{\frac{3}{2}} + \sigma^2\frac{9}{[2\xi-6\phi]^2(t+3)}\\
\end{eqnarray*}

This leads us to the final theorem. To obtain Theorem \ref{minmaxtheorem_appendix}, we proceed in an analogous way as form Theorem \ref{maxmaxtheorem_appendix}, but this time applying Theorem \ref{convergence_2} that we have just proved.
